# Supplementary material for: Reliability and comparability of human brain structural covariance networks
Source: arXiv:1911.12755 source file (2020-05-28)
Supplement: Supplementary file 1 [file Supplementary_v3.pdf]

# Supplementary materials for: Reliability and comparability of human brain structural covariance networks

Jona Carmon[a], Jil Heege[b], Joe H Necus[c,d], Thomas Owen[c], Gordon Pipa[a], Marcus Kaiser[c,d,f], Peter N Taylor[c,d,e], Yujiang Wang[c,d,e,*]

[a] *Institute of Cognitive Science, Osnabrueck University, Osnabrueck, Germany*
[b] *Humboldt University Berlin, Berlin, Germany*
[c] *Interdisciplinary Complex Systems Group, School of Computing, Newcastle University, Newcastle upon Tyne, UK*
[d] *Institute of Neuroscience, Faculty of Medical Sciences, Newcastle University, Newcastle upon Tyne, UK*
[e] *Institute of Neurology, University College London, UK*
[f] *School of Medicine, Shanghai Jiao Tong University, Shanghai, China*

---

---

## Contents

**1 Site comparison on additional network measures** **2**

**2 Mean correlation strength is lowest in average cortical thickness** **4**

**3 Measured correlations compared to estimated corrected correlations** **6**

**4 Larger estimated underlying correlations are less attenuated** **8**

**5 Relationship of estimated error, attenuation and reliability on HCP rescan data** **11**

**6 Relationship of estimated error, attenuation and reliability on Can-CAN FreeSurfer 6.0** **13**

**7 Relation of estimated error, attenuation and reliability on Can-CAN FreeSurfer 5.3** **14**

**8 Estimated true correlations and error structures are a reasonable fit for our simulated data** **15**

*Corresponding author
*Email address:* `yujiang.wang@ncl.ac.uk` (Yujiang Wang)

**9 Test of the estimated corrected correlation** **16**

**10 Reliability and comparability by ROI volume** **18**

**11 Spearman's correlation coefficient results** **20**

**12 Coefficient of variation is smallest in average cortical thickness by a magnitude of 5** **22**

**13 Comparability and reliability brain surface heatmaps for all brain measures** **24**

**14 Scan-rescan differences for shorter inter-session intervals** **25**

**15 Difference in structural covariance for different image resolutions** **27**

**16 Site comparison between Cam-CAN (FS 5.3) and NKI** **29**

**17 Site comparison for Cam-CAN (FS 6.0) and NKI** **31**

**18 Effect of number of subjects on comparability** **33**

**19 Effect of number of subjects on reliability** **35**

## 1. Site comparison on additional network measures

Fig. 4 in the main manuscript showed significant difference for the $L_1$ distance and other network measures. Here, we used the same data as in Fig. 4(A) and added additional network measures.

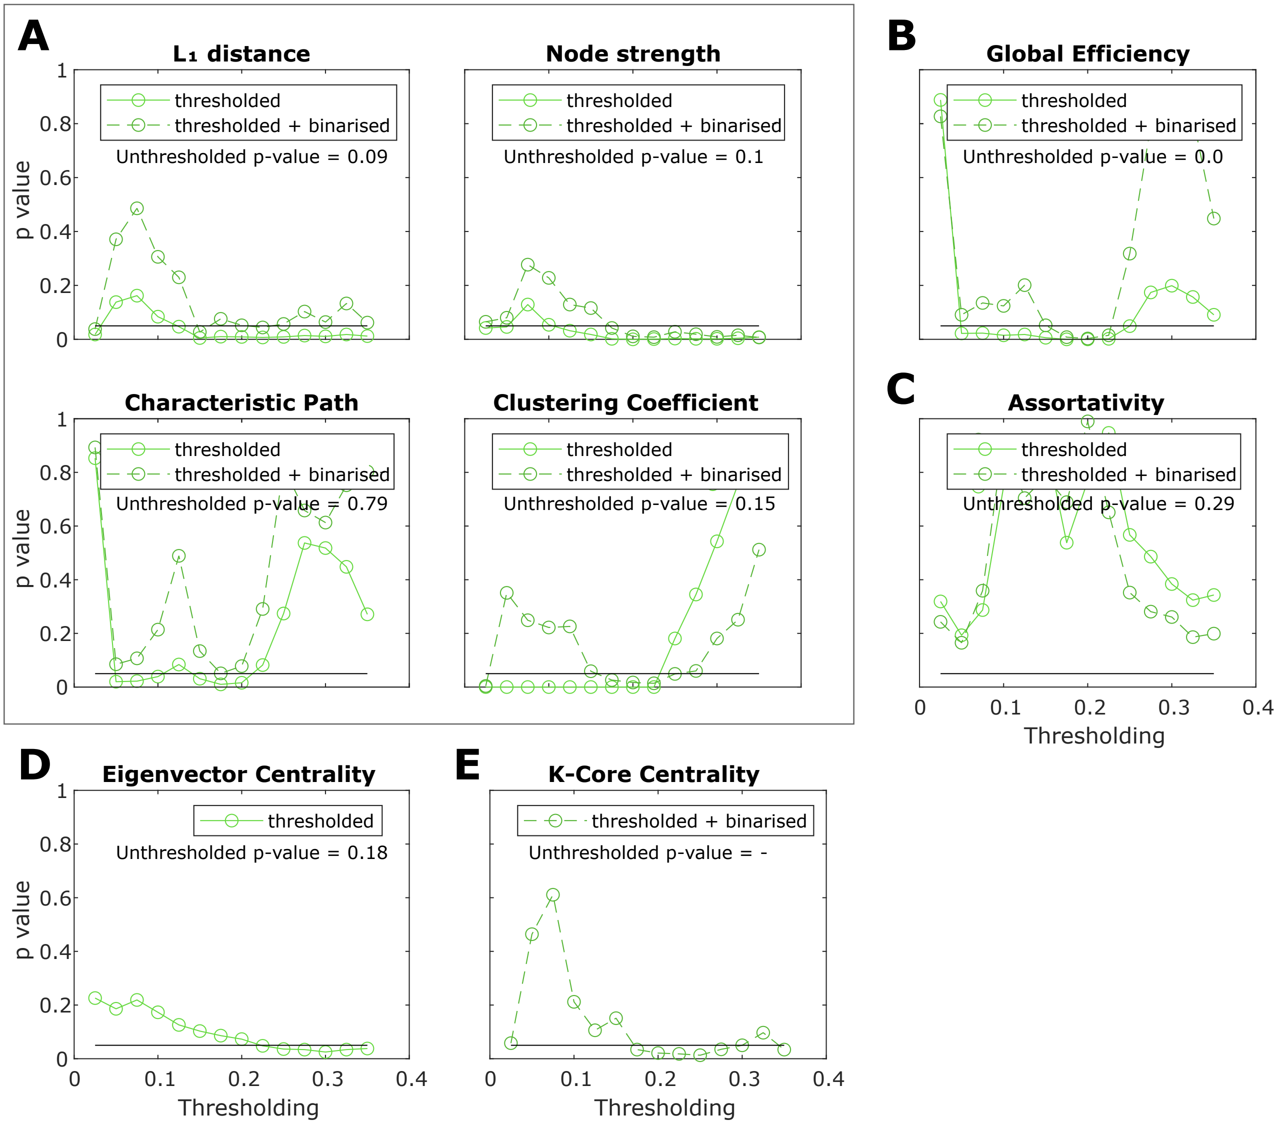


Figure S1: Panel (A) shows the $L_1$ distance and the comparison of network measures depicted in Fig. 4. Panel (B) - (E) show the comparison of additional network measures. The solid line corresponds to the thresholded matrix comparison and the dashed line corresponds to the thresholded and binarised matrix comparison. The y-axis depicts the p-value of the comparison. Underneath the legend is the p-value of the not thresholded and not binarised matrix comparison displayed.

We can see in Fig. S1 that there are also significant differences for the additional network measures. Assortativity is the only exception.

In summary, additional network measures also show significant differencec in structural covariance of cortical thickness between Cam-CAN and HCP.

## 2. Mean correlation strength is lowest in average cortical thickness

In Fig. 6(A) in the main manuscript we could see that the correlation of the left and right hemisphere is lower for thickness compared to volume and surface area. Here, we investigated if this extends to the correlations of ROIs in the Desikan-Killiany atlas. We display the correlation strengths of each measure in a boxplot.

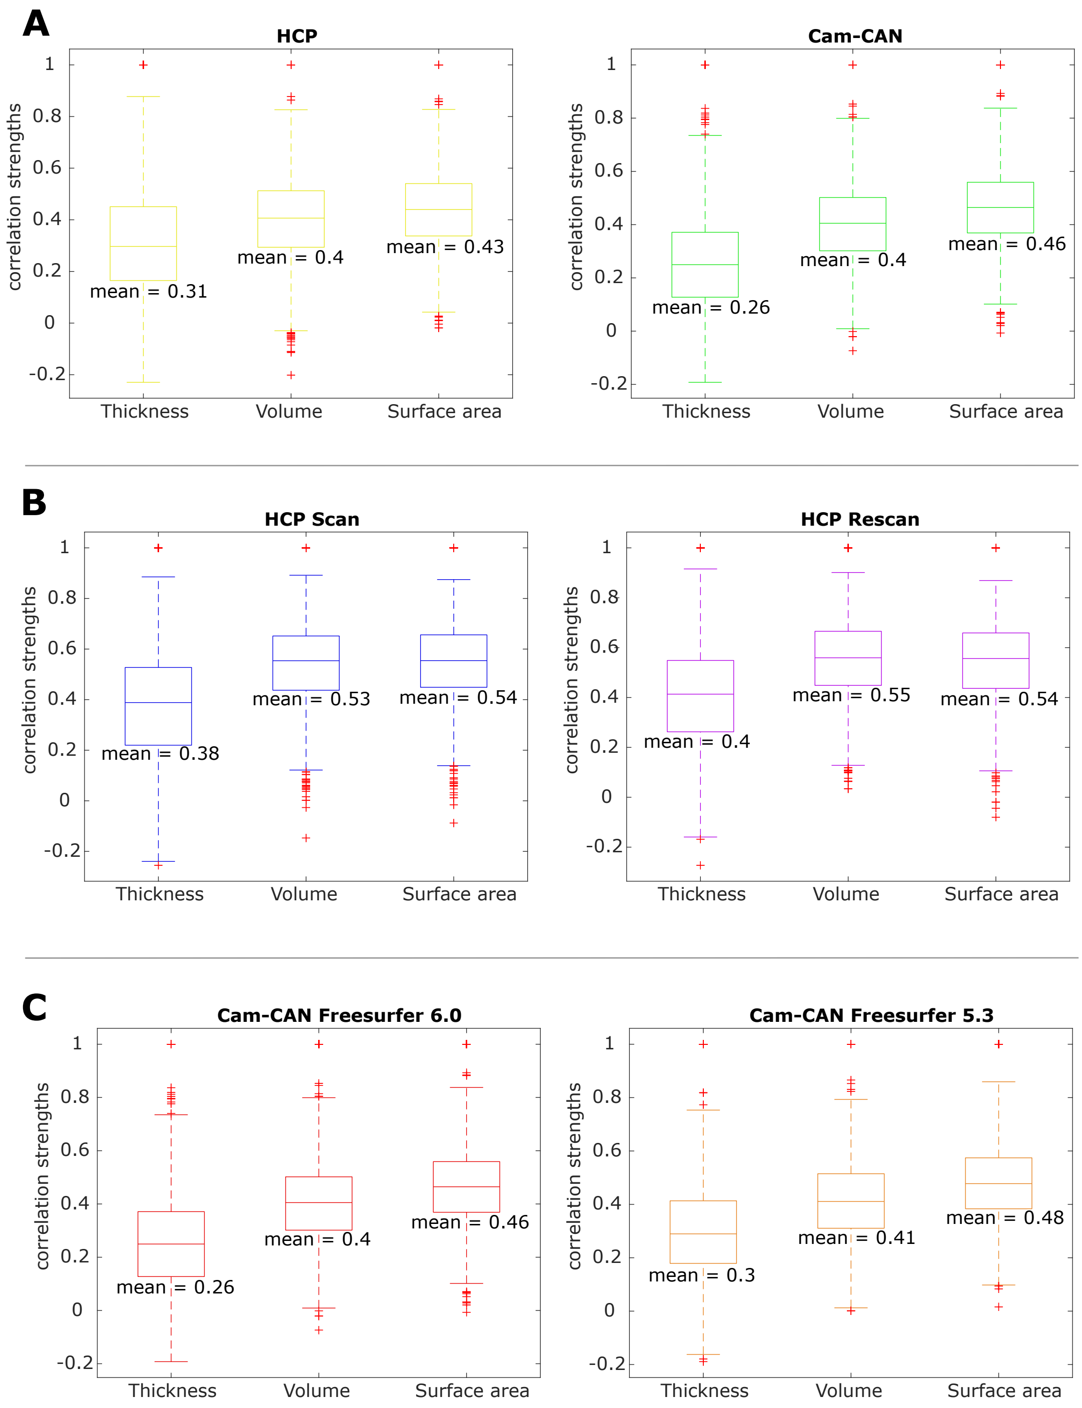


Figure S2: All panels show the correlation strength of thickness (left), volume (middle) and surface area (right). Panel (A) shows the correlation strength of HCP (yellow) and Cam-CAM (green), panel (B) the correlation strength of the HCP scan (blue) and rescan (purple) data, and panel (C) the correlation strength of Cam-CAN FreeSurfer version 6.0 (red) and FreeSurfer version 5.3 (orange)

We can see in Fig. S2 that the mean and median correlation strength is clearly smaller in thickness compared to volume and surface area. For most of our data sets the correlation of volume is smaller than the correlation of area, but this difference is less distinct. For the scan and rescan data the correlation strength of volume and area is almost identical. Thickness has more negative correlations than the other cortical measures. But the mean and median correlation strength is also smallest in thickness when taking the absolute value of the correlations.

In summary, our analysis shows that also for the correlations of the Desikan-Killiany atlas the correlations are lowest for thickness. The correlation strength of area and volume is similar, but correlations of area tend to be larger.

## 3. Measured correlations compared to estimated corrected correlations

We could see in Fig. 6 in the main manuscript that all measured correlations are attenuated compared to the estimated corrected correlations. In this analysis we wanted to see if this extends to the correlations of the Desikan-Killiany atlas.

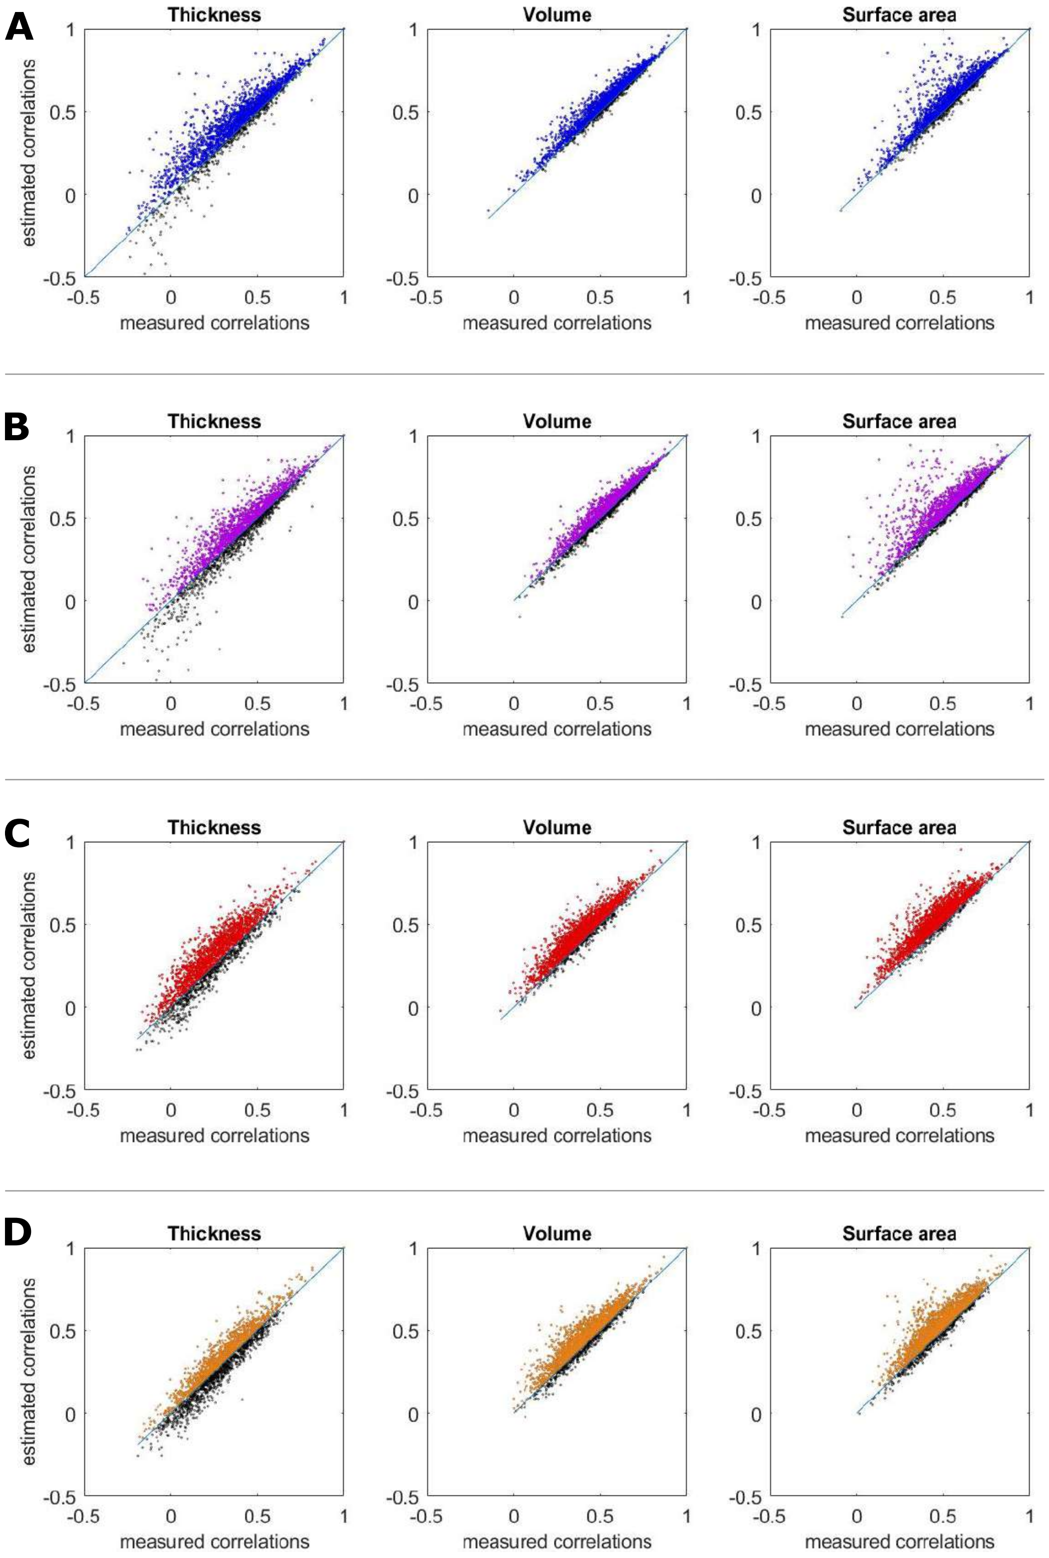


Figure S3: All panels show the measured correlation on the x-axis and an estimated 'true' correlation based on repeat measurements on the y-axis of ROI-pairs from the Desikan-Killiany atlas. The first column corresponds to thickness, the second column to volume and the last column to surface area. We calculated panel (A) with the scan data, panel (B) with rescan data, panel (C) with FreeSurfer version 5.3 and panel (D) with FreeSurfer version 6.0. Attenuated correlations are displayed in color.

For Fig. S3 we used the HCP scan and rescan data as well as the CamCAN FreeSurfer 5.3 and 6.0. We estimated a corrected structural covariance matrix for the scan and rescan data as well as a corrected structural covariance matrix for the FreeSurfer versions. To estimate the corrected structural covariance, we made use of the fact that we have two measurements of all subjects in each data set pair. For details of the calculation and the independence assumptions we made see the methods section. We termed correlations for which the measured correlations are lower than the estimated corrected correlations attenuated.

We can see in Fig. S3 that most correlations are attenuated (coloured). This corresponds to the observation in Fig. 6. For volume and area, almost every measured correlation is attenuated compared to the estimated corrected correlation. In thickness correlations close to 0 and negative correlations are less attenuated. This is especially pronounced for the correlations of FreeSurfer version 5.3.

As expected from Fig. 6 we could show that also for the correlations of the Desikan-Killiany atlas most measured correlations are attenuated compared to the estimated corrected correlations. For most types of error one expects that the corrected correlation is higher than the correlation to which we add error. We would only observe an increase in the empirically measured correlation vs. the estimated corrected correlation in the special case where error of the ROI pair is very correlated, but the cortical morphology is not. Why this appears to be the case for some correlations of thickness is not certain. Future work with multiple repeat measurements maybe better suited to investigate this.

## 4. Larger estimated underlying correlations are less attenuated

In Fig. 5 of the main manuscript we could see that the correlations of thickness are least reliable and comparable. Further, in Fig. 6 and Fig. 7 we showed that less reliable correlations have a stronger estimated error covariance. We also could show that correlations with stronger error are attenuated more and demonstrated the link between attenuation and reliability. Since, the correlations in thickness are least reliable and have the biggest estimated error we would also expect the correlations of thickness to be the most attenuated. Indeed, for the correlation of the left and right hemisphere the correlations of thickness are most attenuated, but for the correlations of the Desikan-Killiany this is not the necessarily the case. Below we investigate a potential explanation of this observation. We know that the measured and the corrected correlations alike are lower in thickness than for the other cortical measures. We hypothesise that lower correlations are attenuated less for the same magnitude of added error.

We used the HCP scan and rescan data and the CamCAN FreeSurfer 6.0 and 5.3 data. With these data sets we computed the structural covariance of the Desikan-Killiany brain atlas. Further, we estimated a corrected structural covariance for the data set pair of scan sessions as well as for the data set pair of FreeSurfer versions. Since we are interested in attenuation, we included

only attenuated correlations (i.e. we only included correlations for which the estimated corrected correlation is larger than the measured correlation).

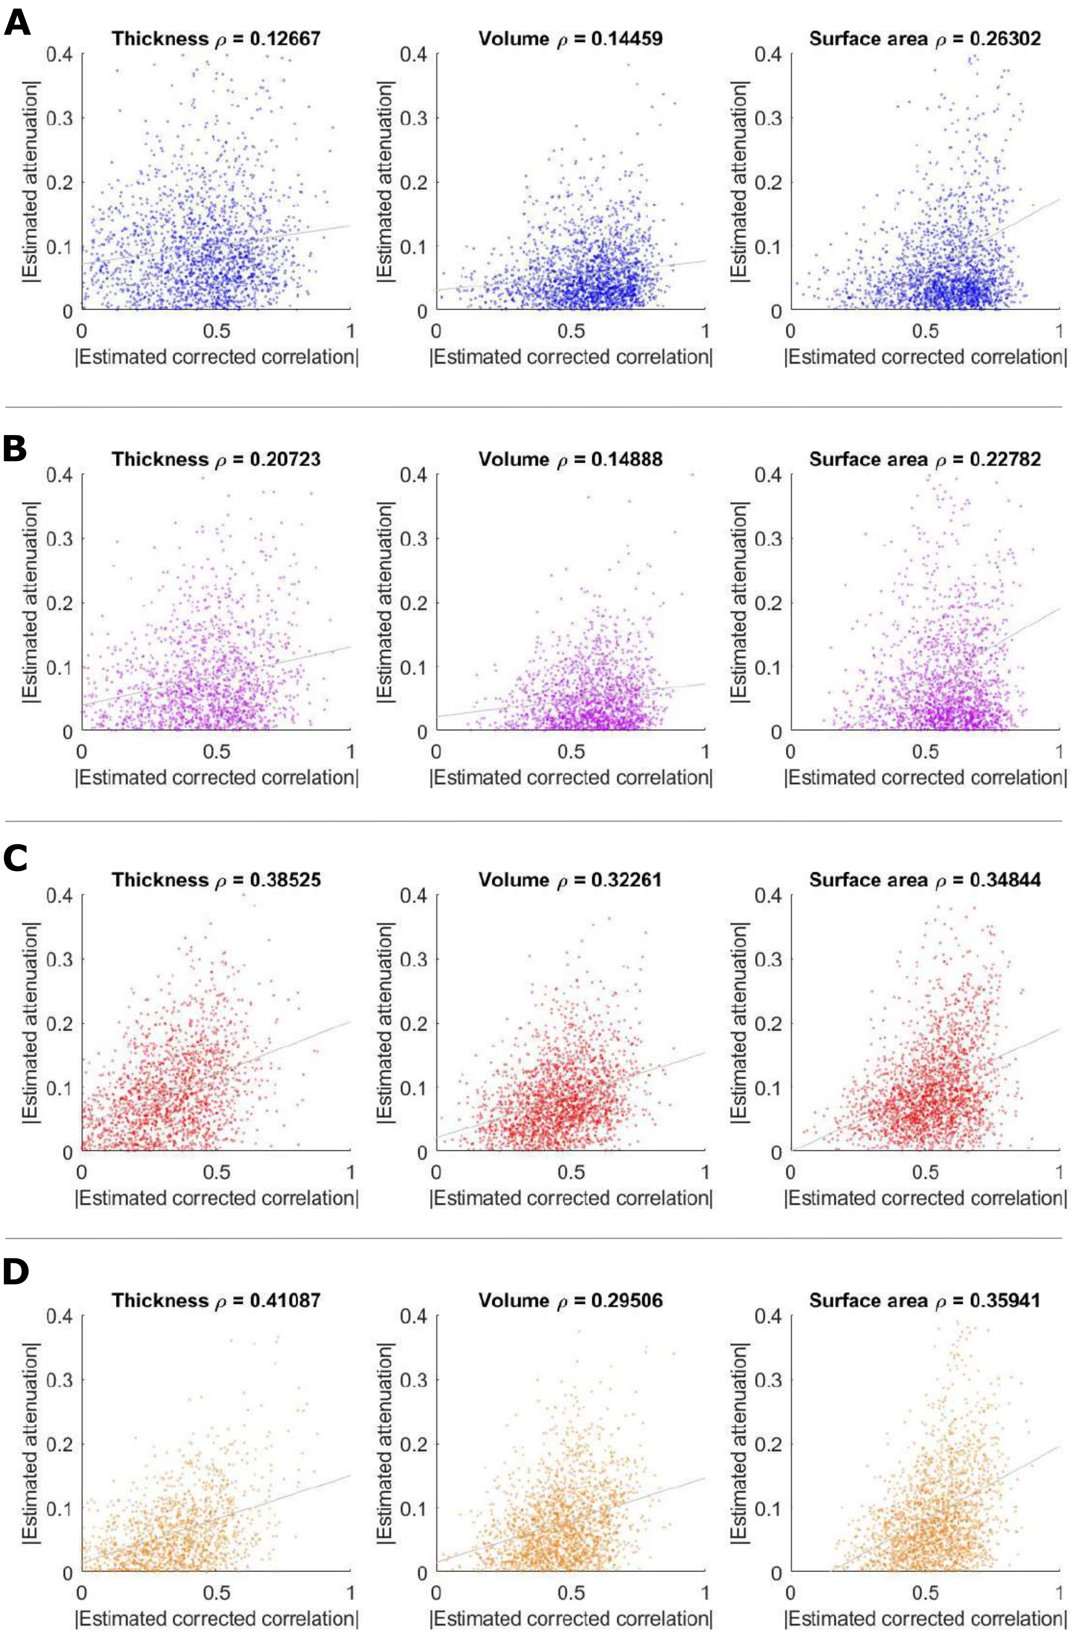


Figure S4: The estimated corrected correlations plotted against the estimated attenuation. We computed panel (A) with the HCP scan data, panel (B) with the HCP rescan data, panel (C) with the FreeSurfer version 5.3 and panel (D) with the FreeSurfer version 6.0. Each column corresponds to one cortical measure.

In all panels in Fig. S4 we can see a small positive relationship for lower correlations to be less attenuated than higher correlations. Together with the fact that the corrected correlations are lower in thickness, this gives us a possible explanation why thickness - even if it is affected with a larger relative error (and possibly for this reason is less reliable) - nevertheless is not more attenuated. This finding is also underscored by the simulated data of Fig. 7(A). The simulation shows that for the same error strength lower correlations are less attenuated than larger correlations. The effect of error on reliability seems to be much less affected by the correlation strength.

Why the corrected correlations are lower in thickness in the first place is however uncertain. We presume the corrected correlations to be lower, because we correct the correlation in our work only for one error source (either scan session or FreeSurfer version). However, we can expect that also in preceding processing steps thickness is more prone to error and potentially already more attenuated than the other cortical measures. Alternatively, the true biological correlation might be lower for thickness.

## 5. Relationship of estimated error, attenuation and reliability on HCP rescan data

We used the HCP scan data for panels (B)-(D) of Fig. 7 in the main results. Here, we reproduced these panels with the HCP rescan data (Fig. S5), Cam-CAN FreeSurfer 5.3 (Fig. S6) and Cam-CAN FreeSurfer 6.0 (Fig. S7).

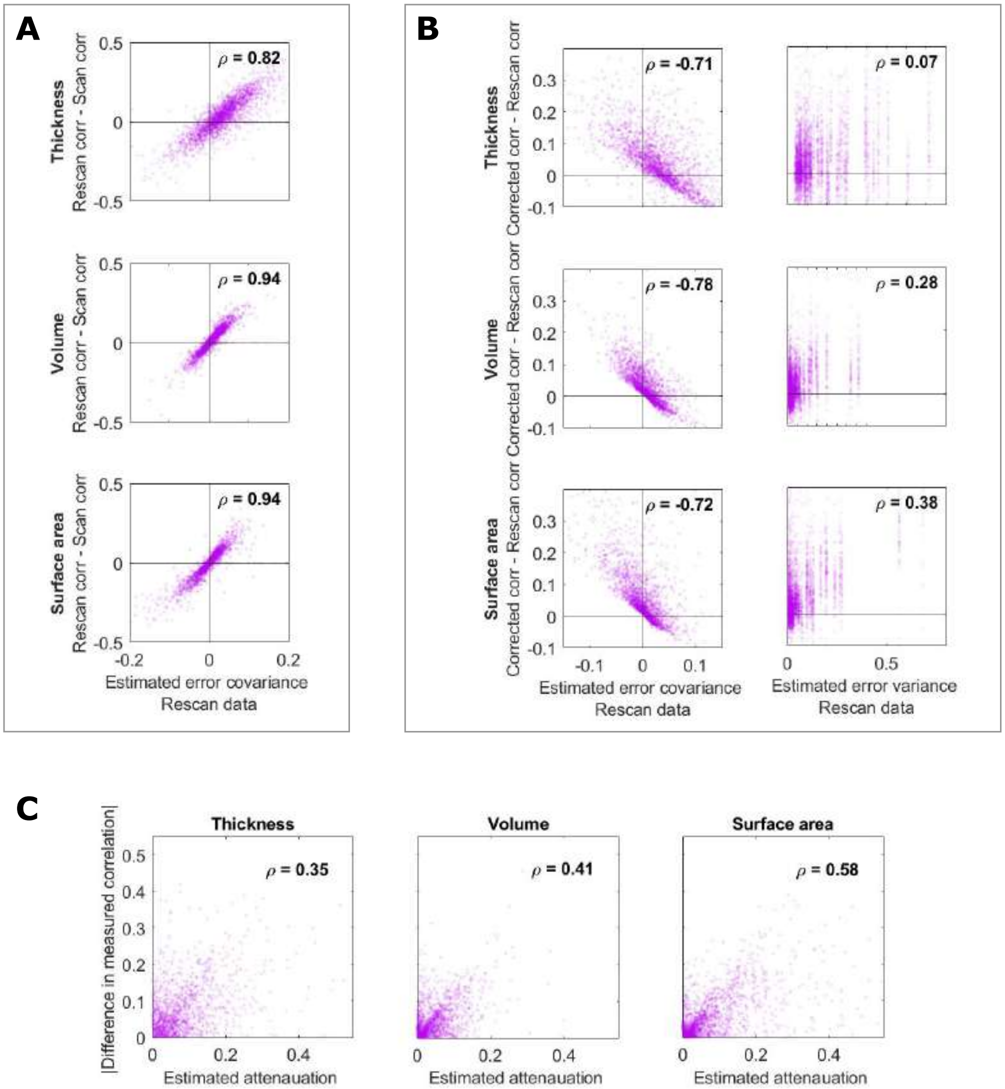


Figure S5: (A)-(C) use HCP rescan data. (B) shows the estimated error covariance scattered against the measured correlations of HCP rescan data minus measured correlations of HCP scan data. (C) shows the estimated covariance error (left column) and estimated variance error (right column) scattered against the estimated 'corrected' correlation minus the measured correlation (HCP scan data). (D) displays the estimated attenuation scattered against the absolute difference in measured correlations

We can see that the computations of these data sets also result in very similar plots like of Fig. 7. Fig. S7: For thickness the correlation of the variance and the difference of estimated corrected correlation minus measured correlation is close to 0. Also, in all three cortical measures the correlations of attenuation and the difference in measured correlations is lower than for the other data sets.

In summary, we could show that the observations on the HCP scan data of Fig. 7 in the main manuscript also extend to the other data sets.

## 6. Relationship of estimated error, attenuation and reliability on Can-CAN FreeSurfer 6.0

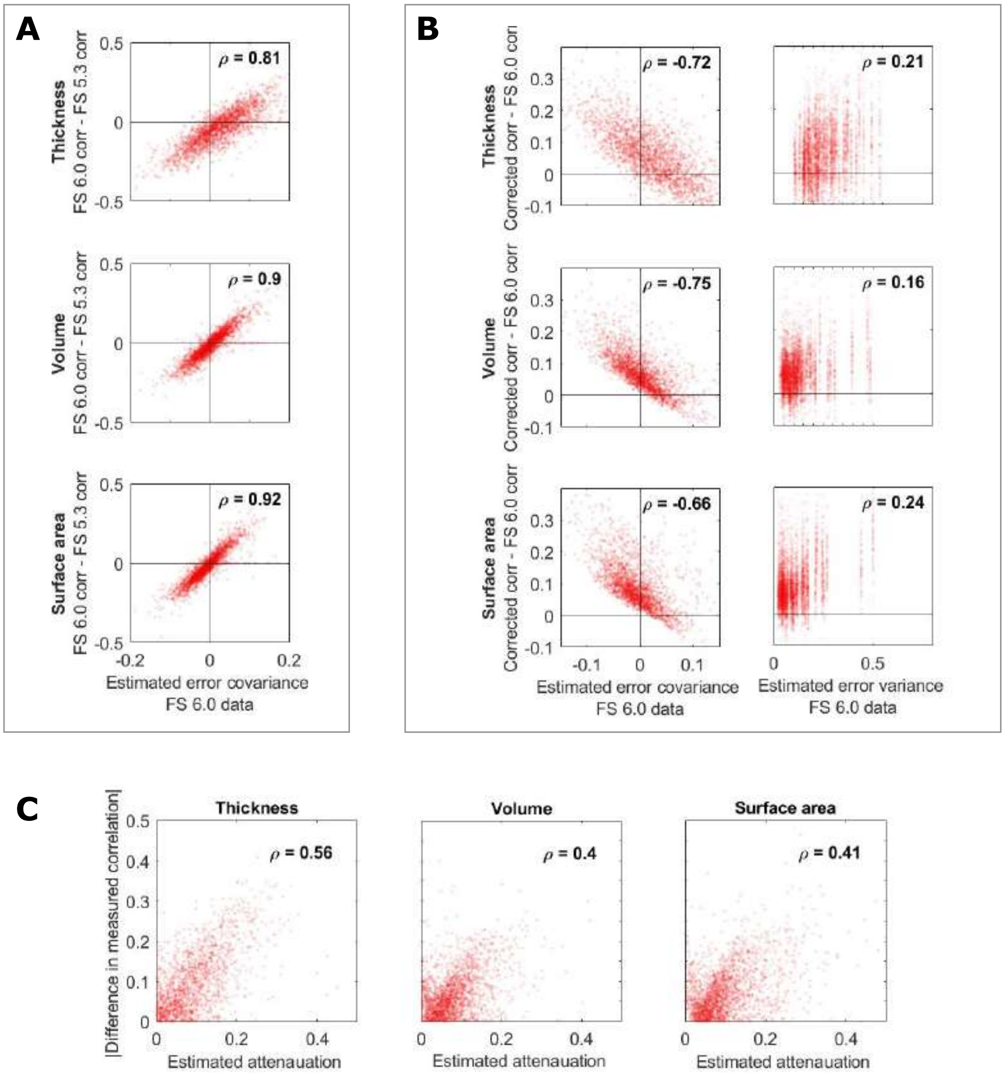


Figure S6: (A)-(C) use Can-CAN FreeSurfer 6.0 data. (B) shows the estimated error covariance scattered against the measured correlations of Can-CAN FreeSurfer 6.0 data minus measured correlations of Can-CAN FreeSurfer 5.3 data. (C) shows the estimated covariance error (left column) and estimated variance error (right column) scattered against the estimated 'corrected' correlation minus the measured correlation (FreeSurfer 6.0 data). (D) displays the estimated attenuation scattered against the absolute difference in measured correlations

## 7. Relation of estimated error, attenuation and reliability on Can-CAN FreeSurfer 5.3

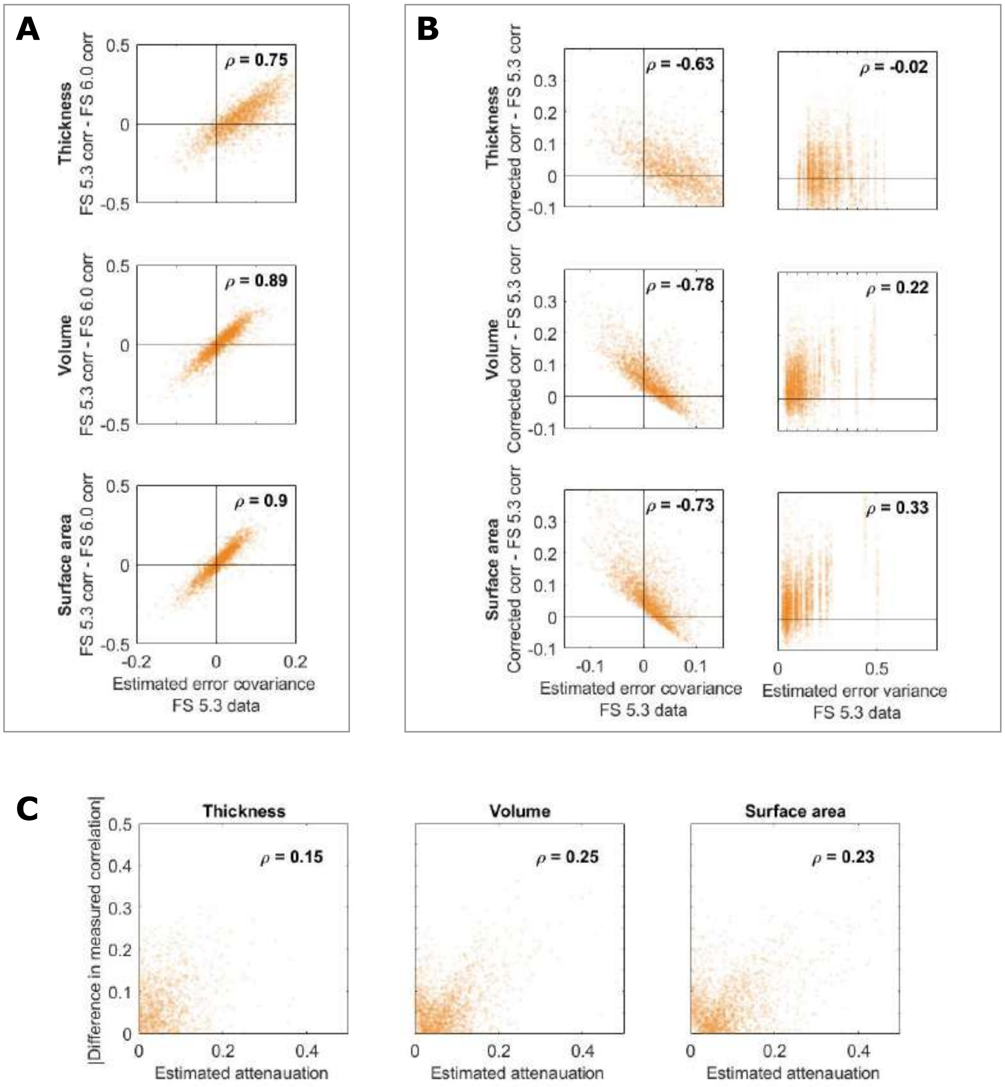


Figure S7: (A)-(C) use Can-CAN FreeSurfer 5.3 data. (B) shows the estimated error covariance scattered against the measured correlations of Can-CAN FreeSurfer 5.3 data minus measured correlations of Can-CAN FreeSurfer 6.0 data. (C) shows the estimated covariance error (left column) and estimated variance error (right column) scattered against the estimated 'corrected' correlation minus the measured correlation (Can-CAN FreeSurfer 5.3 data). (D) displays the estimated attenuation scattered against the absolute difference in measured correlations

## 8. Estimated true correlations and error structures are a reasonable fit for our simulated data

In panel (A) of Fig. 7 in the main text, we investigate the effect of error on attenuation and reliability on the simulated data. Further, in panel Fig. 7(B)-(D) in the main text, we could show that our results of the simulation go in line with observations on the real data. Here, we wanted to see if, on simulated data, our estimates of the true correlation are close to the actual values and our estimated error variance and covariance reflect the relative errors.

In order to compute the corrected correlation and error variance and covariance we need two measurements of every correlation. Therefore, we generated two versions of every measurement. We created each version by an independent noise vector.

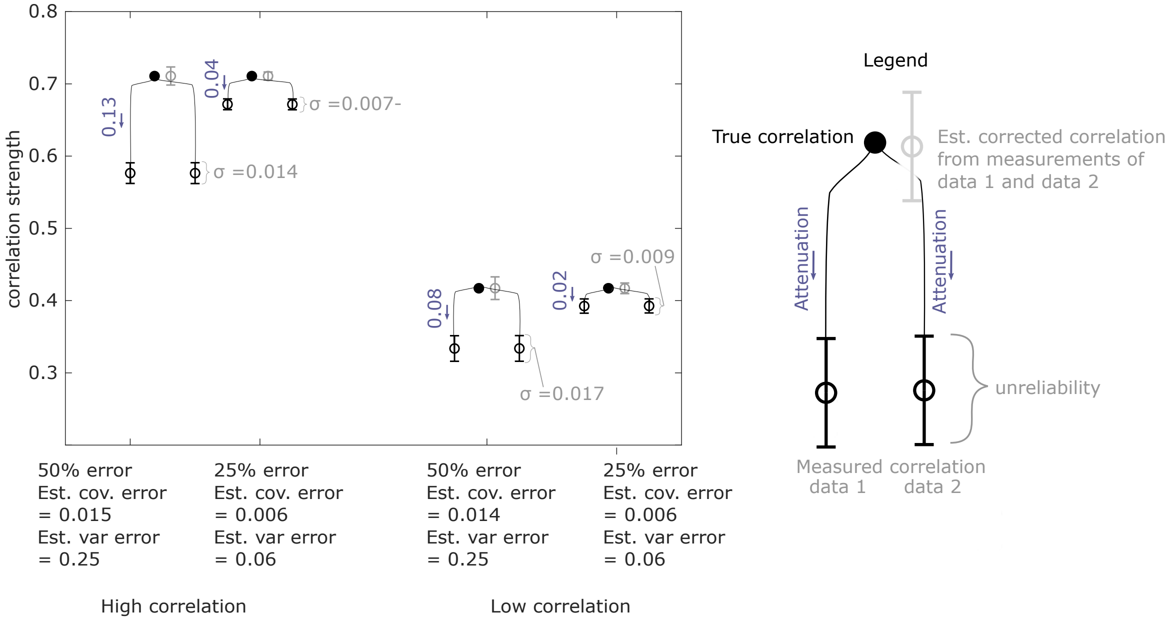


Figure S8: Testing our estimates for Fig. 7's simulation on artificially generated data. Unlike in Fig. 7(A) we have two measurements of every correlation. This let us estimate the corrected correlations (in grey).

We can see in Fig. S8 that the estimated true correlation reflects the actual true correlation well. The variation of the estimated true correlations is similar to the respective variation of the measured correlations.

Further, we can see that for the same error strength the estimated error covariance and variance are roughly the same regardless of the correlation strength to which we added the error.

In summary, the estimates seem to be a good fit for our simulation of Fig. 7. This supports that it is reasonable to relate our simulation to our real data.

## 9. Test of the estimated corrected correlation

Part of our work relies on an estimate of corrected correlations based on repeat measurements. Here, we wanted to test how well our estimate reflects the true underlying correlation on an artificially generated data set and see if it is closer to the true correlation than the measured correlations.

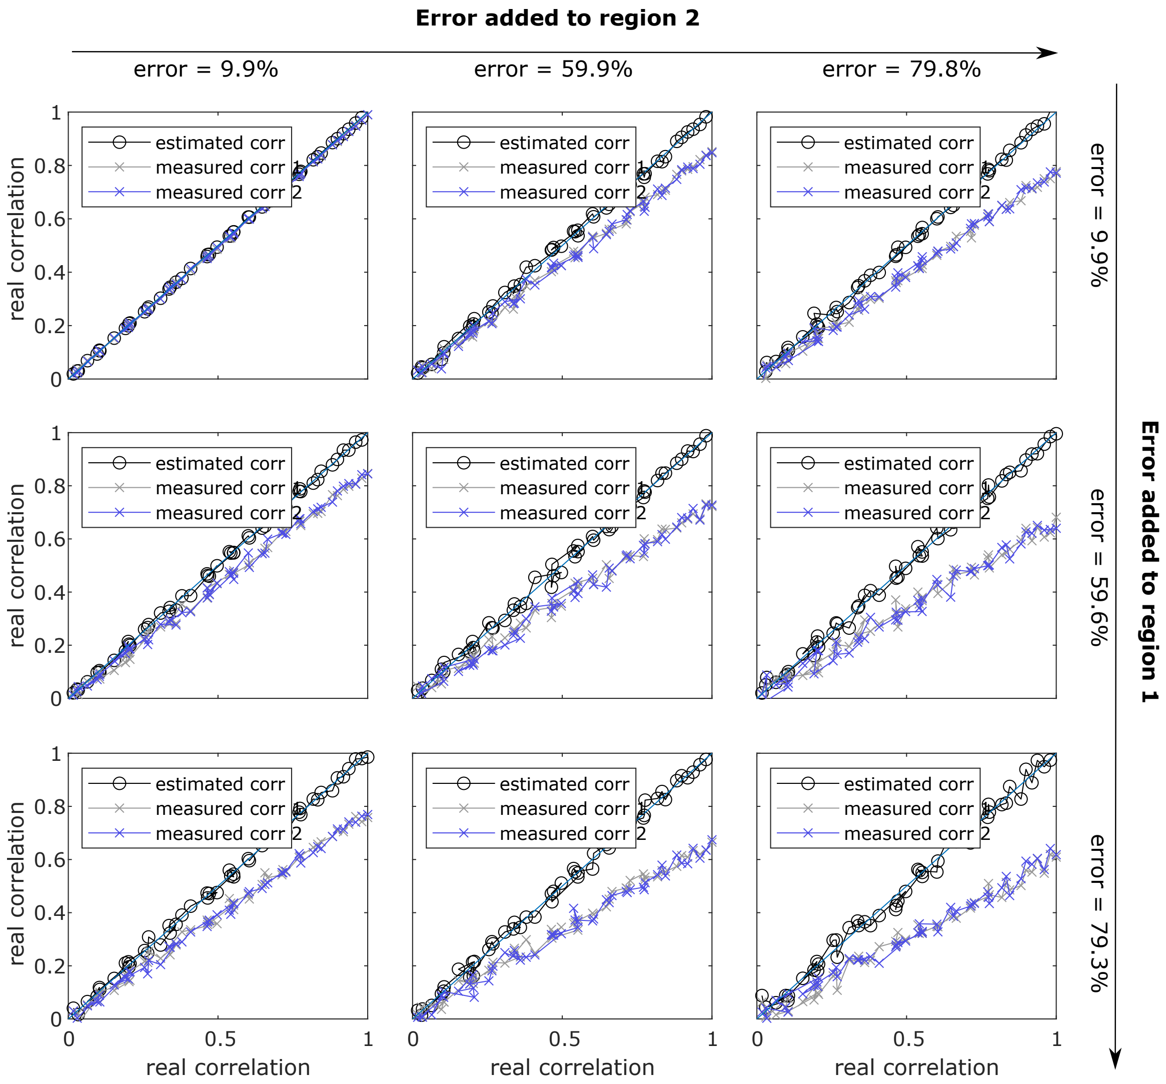


Figure S9: Test of the estimated corrected correlation value. The solid line displays the real correlation value, the grey and blue line the measured correlations and the black line the estimated corrected correlation. The error added to region 1 increases between the panels in y-direction and the error added to region 2 increases between the panels in x-direction.

We generated a data set of two variables. Each of the variables could correspond to one brain region. We computed 50 different versions of these variables from strongly correlated to not correlated at all. This allows us to test our estimate for the whole range of correlation strengths. To simulate two measurements (like scan sessions or FreeSurfer versions) we added measurement error

to the generated data independently. The panels in Fig. S9 show an increase of this added error to the first variable (first brain region) on the y-axis and an increase of the added error to the second variable (second brain region) on the x-axis.

For increasing error (in x and y direction), we can see that the measured correlation decreases. Our estimated corrected correlation is clearly closer to the underlying true correlation especially for higher error levels. Our simulation also shows that stronger correlations are clearly more attenuated than lower correlations for the same error level.

In summary, this simulation shows that our estimated correlation predicts the underlying correlation well for all correlation strengths. It is clearly closer to the true correlation than the measured correlations and yields reasonable results up to a high level of error. It also shows that higher correlations are attenuated more for the same amount of error, which go in line with other parts of our work (Fig. 7(A) and Fig. S4). In how far the generated data set reproduces properties of our real data should be investigate in future work.

## 10. Reliability and comparability by ROI volume

An interesting question for our study is if more reliable and comparable ROIs share common features. In this analysis we were interested if the ROI's volume stands in relation to its reliability and comparability.

Here, we analysed the same data sets as in the main results (HCP and Cam-CAN, scann sessions and FreeSurfer versions). We used the Desikan-Killiany atlas, and computed a p-value for each ROI pair between the comparison sets. From that we computed the mean p-value per ROI. Further, we computed the mean volume for each ROI (on CamCAN site, scan data, and FreeSurfer 6.0, respectively).

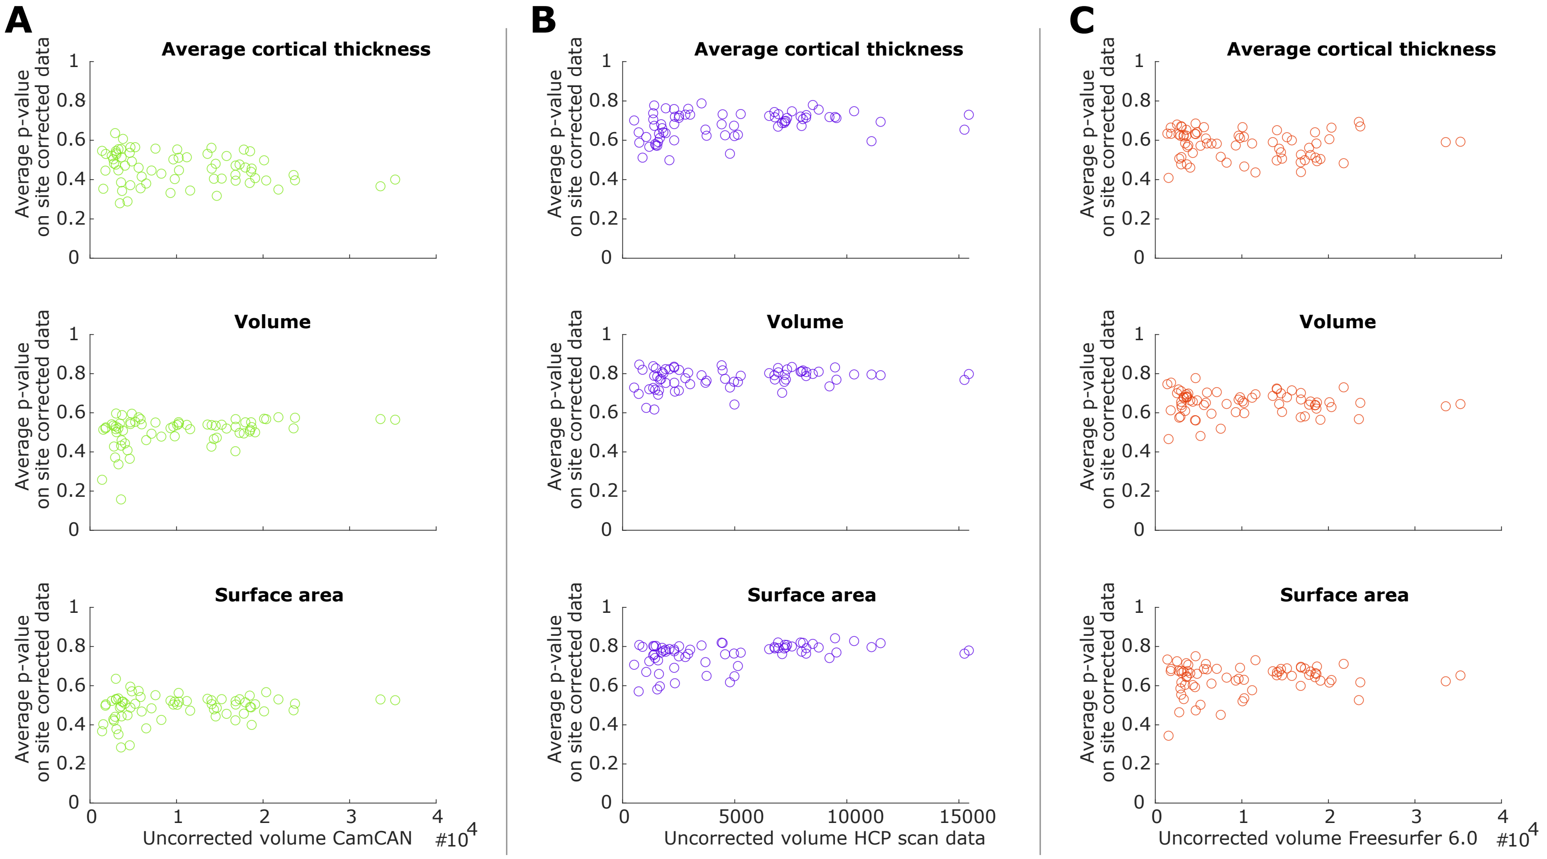


Figure S10: The mean ROI p-value of site, scan/rescan, and FreeSurfer version comparison scattered against mean ROI volume. Panel (A) show the site comparison of HCP and CamCAN, panel(B) the comparison of HCP scan and rescan and panel (C) the comparison of the FreeSurfer versions.

We can see in Fig. S10 that there is a higher variance of p-values for smaller ROIs. The p-values of smaller ROIs also tend to be smaller or equal to the p-value of larger ROIs. We can also observe that the p-values of the site comparison of HCP and CamCAN are lower than the p-values of comparisons of scan sessions and FreeSurfer versions.

Our analysis showed a slight difference in ROIs p-value according to their volume. Smaller ROIs show a bigger variance in p-value and can be less reliable. A larger size may increase the measurement to error ratio and therefor yield

better reliability. Future work can investigate this further for different brain atlases.

## 11. Spearman's correlation coefficient results

To investigate if Spearman's correlation improves the reliability and comparability, we reproduced Fig. 5 from the main results with the Spearman's correlation coefficient. The Spearman's rank correlation is less prone to outliers and we were interested if this has also an effect on the reliability of the covariance structure.

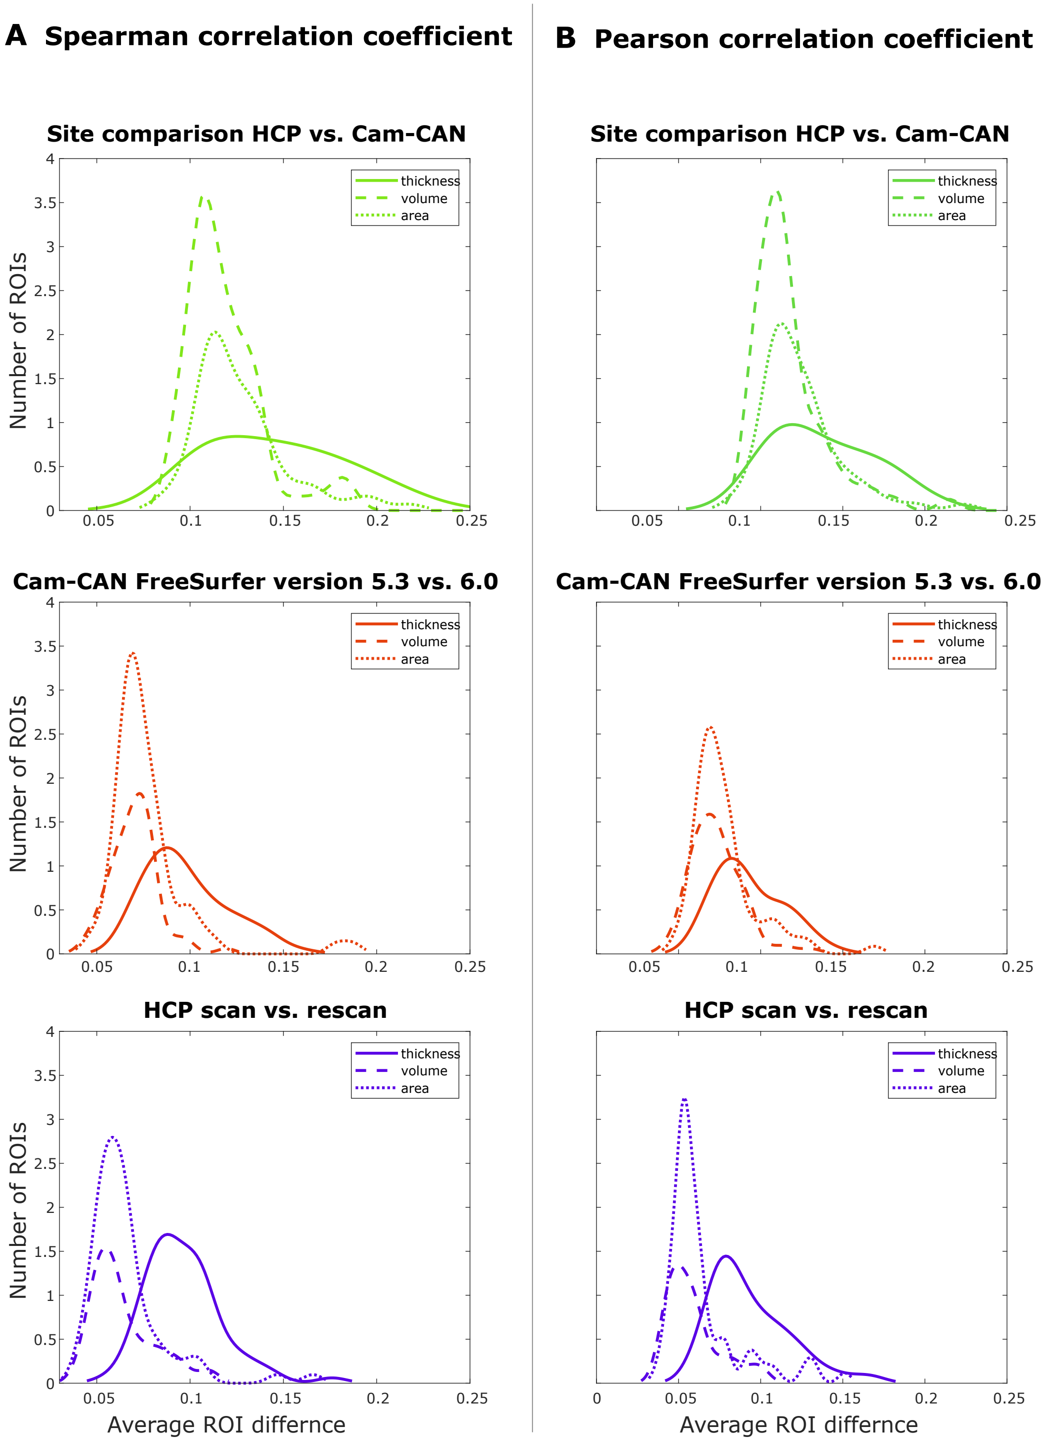


Figure S11: Difference in correlation compared between cortical measures and correlation types. Panel (A) corresponds to correlations computed using Spearman's correlation coefficient. Panel (B) corresponds to correlations computed using Pearson's correlation coefficient. The first row shows the difference in correlation between HCP and CamCAN, the second row between scan sessions and the last row between FreeSurfer versions. The solid line corresponds to thickness, the dashed line to volume and the dotted line to surface area.

We used the same data sets as for Fig. 5 in the main manuscript and computed the same quantities. The only change we applied is that we swapped Pearson's correlation coefficient in the correlation matrix for the Spearman's correlation coefficient. We can see in Fig. S11 that the use of Spearman's correlation coefficient do not change our results substantially, and distribution shapes appear to be similar between the correlation types. We can still see that average cortical thickness is the least reliable of the cortical measures.

In summary, the Spearman's correlation coefficient did not improve the comparability and reliability in our study. This argues for measurement errors driving the main results of low reliability and low comparability.

## 12. Coefficient of variation is smallest in average cortical thickness by a magnitude of 5

It is known that cortical thickness has a lower level of biological variance compared to surface area and volume. Here, we showed that this is also the case for our data sets.

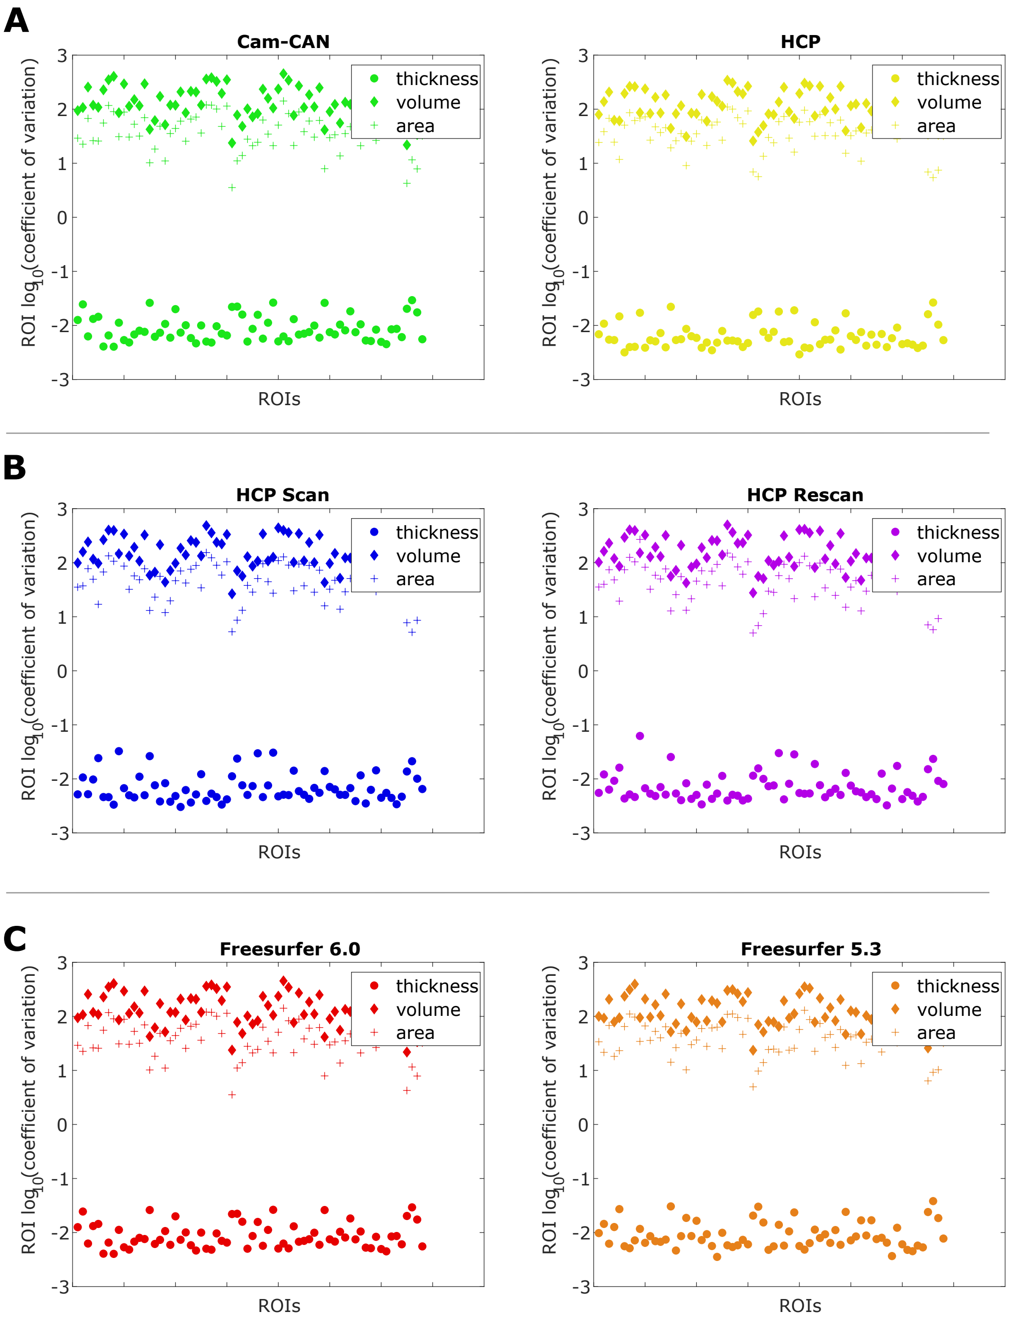


Figure S12: Coefficient of variation compared between different cortical measures. (A) Coefficient of variation of Cam-CAN and HCP. (B) Coefficient of variation of HCP scan and rescan. (C) Coefficient of variation of FreeSurfer version 6.0 and 5.3. measures of thickness are displayed as a circle, measures of volume as a rhombus and measures of area as a +. The coefficient of variation is displayed on a log scale.

In Fig. S12 we can see in all data sets that the coefficient of variation is smallest in average cortical thickness by approximately a magnitude of 5. The

coefficient of variation in volume is slightly larger than in area.

We showed that, also in our data, the coefficient of variation is clearly lower in thickness than volume and surface area. We believe that because of the lower coefficient of variation in thickness, measurement error has a stronger effect. Indeed, we found a stronger relative error in this cortical measure (see e.g. Fig. 6).

## 13. Comparability and reliability brain surface heatmaps for all brain measures

In Fig. 5 of the main results we show a quantification of the difference in reliability and comparability between brain measures. In order to additionally visualise these differences here we also show a heatmap for the site comparison, the scan sessions and the FreeSurfer versions for each brain measure (Fig. S13).

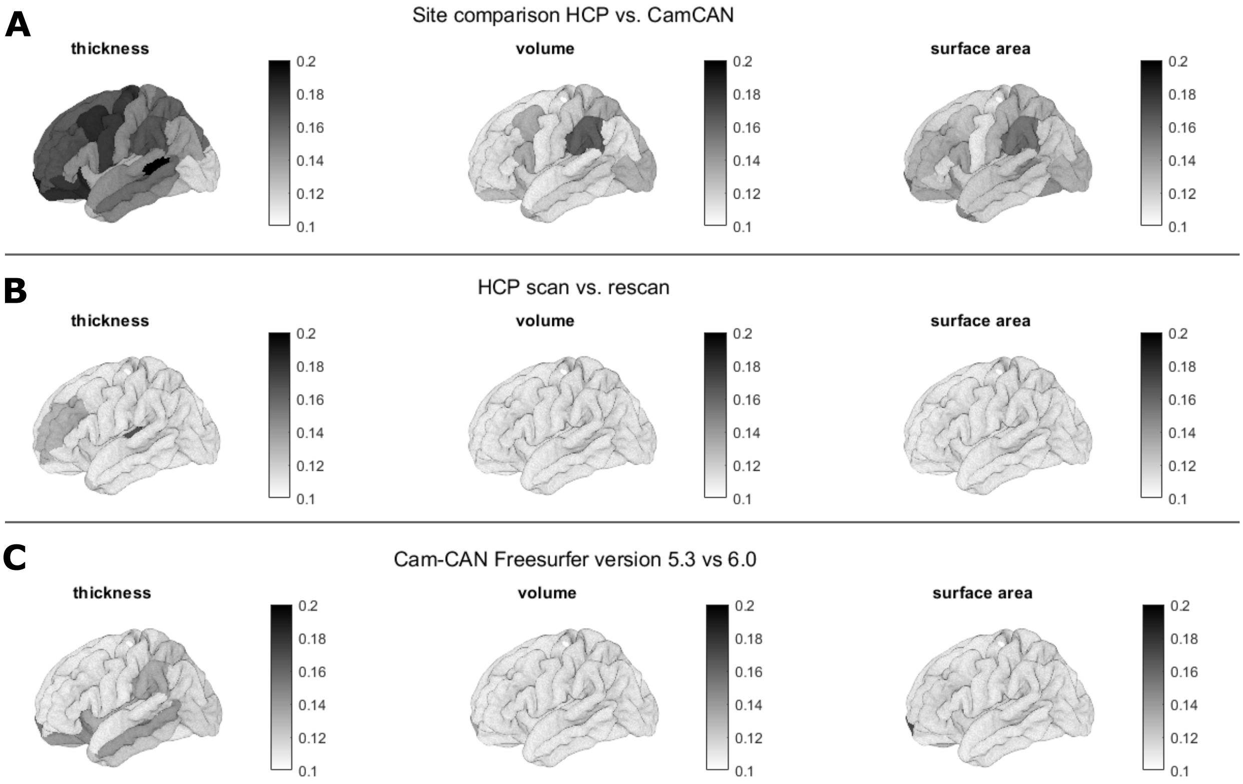


Figure S13: Comparability and reliability brain surface heatmaps for all brain measures. (A) shows the brain heat maps for measures of the site comparison of HCP and Cam-CAN. (B) and (C) display the heatmaps of all measures for differences in scan sessions and FreeSurfer versions, respectively

We can see in Fig. S13 that the differences in thickness are more pronounced than in the other measures. Additionally, the differences of the site comparison are stronger than for the scan sessions or FreeSurfer version comparisons. This leaves the strongest difference in the site comparison of average cortical thickness (Fig. S13(A) on the left).

In summary, these visualisations of the brain heatmap accompany Fig. 5 of the main results and aid our understanding in terms of the difference between different brain measures in terms of reliability and comparability.

## 14. Scan-rescan differences for shorter inter-session intervals

In the main results we show that there are distinct differences between the structural covariance of scan and rescan sessions. We demonstrate this with the HCP scan and rescan data set. However, the scanning interval between HCP scan and rescan is up to two years. Here, we were interested if for a much shorter scan interval the differences in the covariance structure will be reduced. Therefore, we use the Beijing Normal University (BNU) data set (`http://dx.doi.org/10.15387/fcp_indi.corr.bnu1`). The data set comprises of healthy adults scanned in an interval of 6 weeks. Data was available for 41 (age range 19-27, and a 20:21 sex balance) subjects in our study.

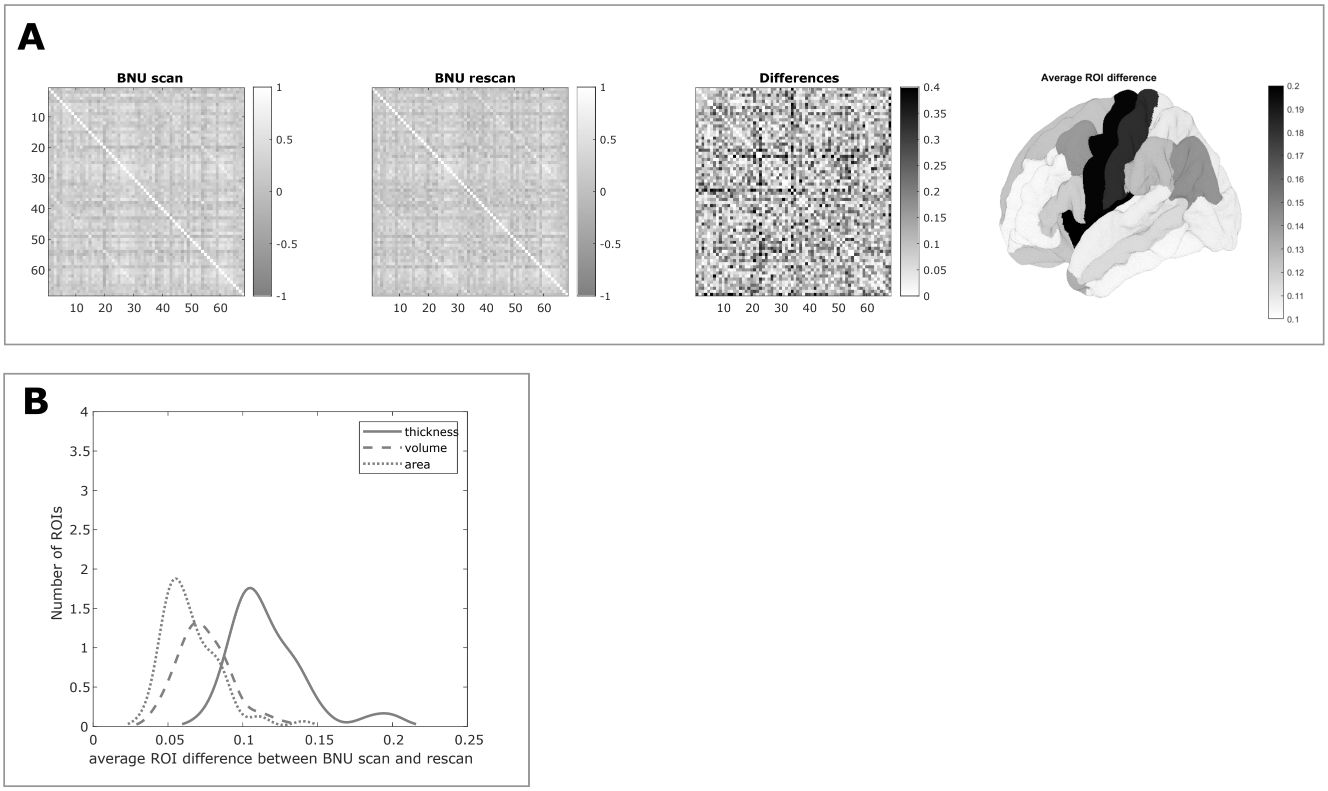


Figure S14: Difference in structural covariance between scan and rescan sessions for shorter inter-session intervals in the BNU dataset. (A) shows the same panel as Fig.3(C) of the main paper. Differences are compared in average cortical thickness. (B) shows the same panel as Fig.5(B) of the main paper. Summary of differences are shown as a distribution for thickness, area, and volume.

Fig. S14(A) shows the difference in the structural covariance such as Fig.3(C) in the main results. Fig. S14(B) shows the histograms of the differences for all three cortical measures as displayed in panel (B) of figure 5 of the main results. For the BNU dataset, as for the HCP dataset, there are differences between scan and rescan sessions in the structural covariance matrix. The differences are not reduced compared to the HCP differences seen in the figures of the main paper. Consistent with all other data sets we can see in Fig. S14(B) that the differences in structural covariance are strongest for average cortical thickness.

Over all, with the BNU data set we can show that the structural covariance differs between scan/rescan sessions, even for a much shorter inter-session interval.

## 15. Difference in structural covariance for different image resolutions

We could show that various factors (e.g. differences in scan session or FreeSurfer versions) can contribute to differences in structural covariance. Another potential factor that could further lead to differences is the resolution of the MR image. The HCP data is acquired at a resolution of 0.7 mm isotropic voxel size. Here, we were interested in how lower resolutions could further affect the structural covariance. Therefore, we downsampled the HCP data (100 unrelated subjects) to a resolution of 1mm, 1.5mm and 2mm. For the preprocessing we used FreeSurfer version 5.3, to be most comparable to the original HCP preprocessed FreeSurfer outputs (a modified version of FreeSurfer 5.3).

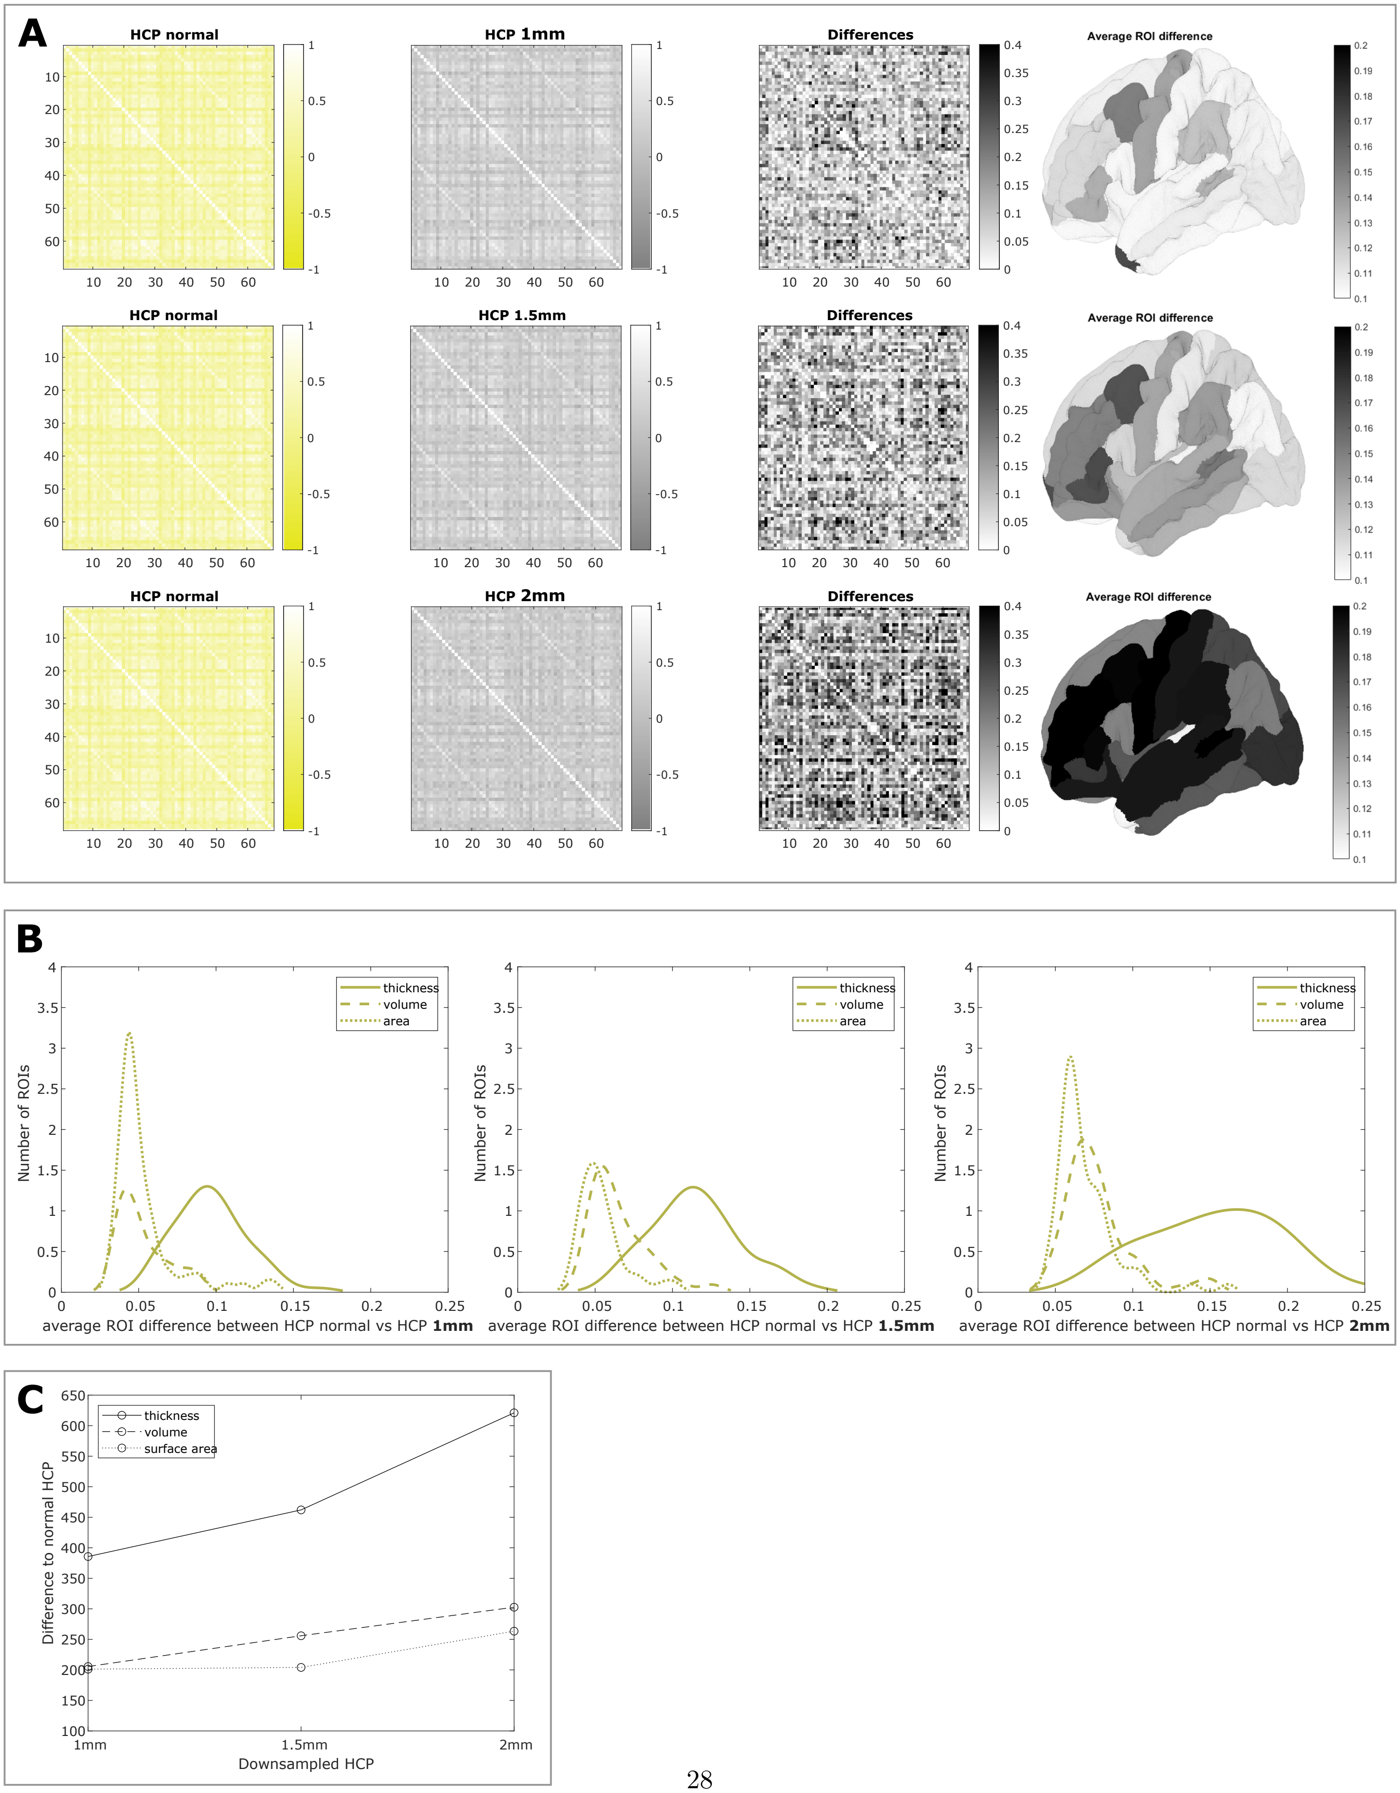




Figure S15: Difference in structural covariance between original HCP image resolution and downsampled versions. (A) and (B) resemble the analyses in figure 3 and 5 in the main text. In both panels, the original HCP dataset is compared to downsampled versions of 1mm, 1.5mm and 2mm. Panel (C) compares the overall differences between the original HCP structural covariance and each of the downsampled versions.

In each row of Fig. S15(A) we show the comparison between the original HCP structural covariance matrix in thickness to a downsampled version (first row 1mm, then 1.5mm and 2mm). Clearly, the difference increases as the resolution is lowered. Panel (B) shows the average ROI difference in structural covariance for all three measures of thickness, area and volume. In line with panel (A) we can also see that the difference increases for lower resolutions. However, the difference increase is less pronounced for volume and area. In the last panel (C), the overall difference between the covariance matrices of the original HCP data and the downsampled versions is shown as a summary.

Our analysis of the reliability between different image resolutions clearly shows its influence on the structural covariance matrix. As expected, the difference in structural covariance increases as the resolution is lowered. Interestingly, the difference in structural covariance between 0.7mm and 1mm isotropic voxel size resolution is approximately as pronounced as the difference between scan/rescan sessions or different FreeSurfer versions (for a comparison see panel (c) and (D) of figure 3 and panel (B) and (C) of figure 5 of the main results). Finally, we can see that for lower image resolutions, one can expect even more distinct structural covariances compared to 0.7 mm isotropic voxel size.

## 16. Site comparison between Cam-CAN (FS 5.3) and NKI

In the main results we compared the HCP and Cam-CAN datasets in terms of their structural covariance. We chose these two data sets as we could find a large number of subject with the same number of males and females in a very narrow age range in both datasets. However, HCP and Cam-CAN differ in the image resolution (0.7mm vs. 1mm isotropic) and in their FreeSurfer setup (for details see methods). Here, we were interested if data sets of the same image resolution and processed using the same FreeSurfer version are more comparable. Therefore, we used the Cam-CAN data set and data obtained from the Nathan Kline Institute (NKI) Rockland Sample [1]. These data sets have the same resolution of 1mm isotropic voxel size. We processed both data sets in FreeSurfer version 5.3. and selected 70 subjects in an age range of 18-48 with the same number of females and males. We had to broaden the age range compared to Cam-CAN and HCP, but still ensured that we had a 1:1 correspondence of subjects in terms of age and sex between the two datasets.

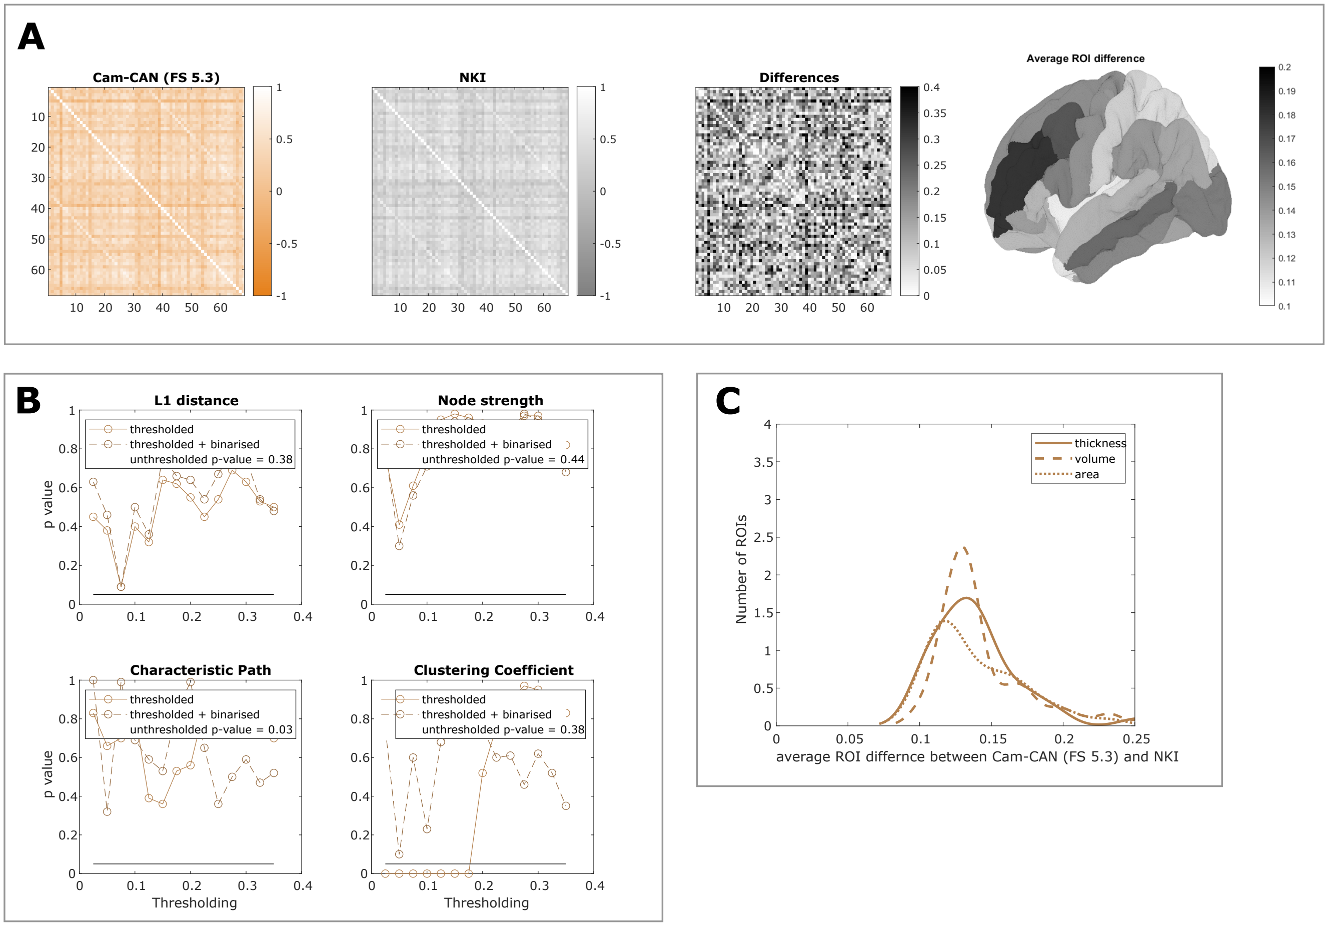


Figure S16: Site comparison between Cam-CAN and NKI, both processed using FS 5.3. All panels are analogous to the panels of the site comparison of figure 3(D), 4(A)-(D) and 5(C) in the main text.

Fig. S16 shows the analogous analysis as the panels for the site comparison of figure 3, 4 and 5 in the main results. Panel (A) shows the structural covariance matrices for the 70 subjects from Cam-CAN and NKI as well as their differences. Clear differences are visible between the structural covariance matrices, which are in a similar range to those in the HCP/CamCAN comparison. The differences are also reflected in the average difference of each ROI, mapped onto the brain surface. Panel (B) shows the p-value of the L1 norm and additional network measures. For the thresholded matrix there are some significant differences for the Clustering Coefficient. For the raw matrix, the differences are significant for the Characteristic Path $p < 0.05$. Panel (C) depicts the average ROI difference for all three brain measures. Unlike in almost all other data set

pairs the average cortical thickness is not clearly least comparable here. The range of differences is comparable to those in the HCP/CamCAN comparison in the main text.

In summary, our additional site comparison shows much less significant differences between the sites. This indicates that the same image resolution and using the same FreeSurfer version for preprocessing improves the comparability. In order to analyse the improvement of comparability from the same FreeSurfer version we compare next NKI with CamCAN preprocessed with a different FreeSurfer version. Although the p-values are mostly comparable nevertheless the matrices are displaying stark differences in structural covariance and we recommend that even generally comparable data sets (with comparable attributes and preprocessing) should not be compared naively.

## 17. Site comparison for Cam-CAN (FS 6.0) and NKI

Additionally, to the comparison above we also compare NKI with Cam-CAN preprocessed with FreeSurfer version 6.0. We were interested if the difference in FreeSurfer versions decreases the comparability.

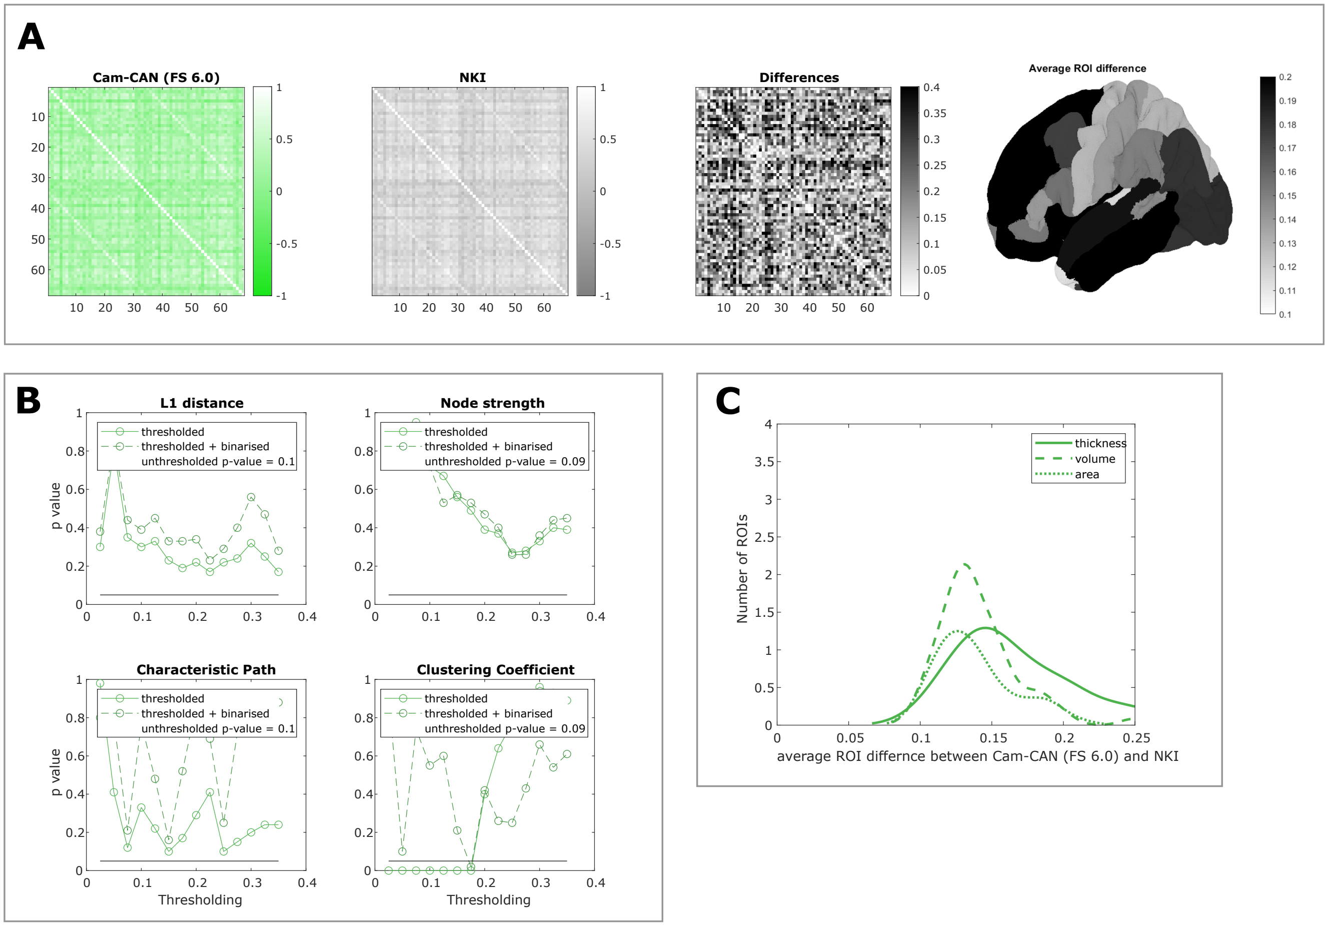


Figure S17: Site comparison for Cam-CAN (FS 6.0) and NKI. All panels are related to the panels of the site comparison of figure 3, 4 and 5 in the main results.

Panel (A) of Fig. S17 shows the structural covariance matrices for the 70 subjects of Cam-CAN and NKI as well as their differences. One can see that clear differences are pronounced between the matrices which can also be seen for the average of each ROI on the heatmap on the brain surface. Panel (B) shows the p-value of the L1 norm and additional network measures. For the thresholded matrix there are significant difference for the Clustering Coefficient. For the unthresholded matrix there are no significant values. Panel (C) depicts the average ROI difference for all three brain meausres. Here, one can clearly see that the differences are stronger than for the comparison of the same FreeSurfer versions.

All in all, we can see that the differences between FreeSurfer versions clearly increase the difference between the structural covariance matrices when com-

pared to the site comparison of the same FreeSurfer versions from above. However, the p-values are not more significant, but overall the p-values might be a little lower.

## 18. Effect of number of subjects on comparability

Here we were interested in if a larger number of subjects would give a improved estimate of the structural covariance matrix and thus also improve comparability and reliability. In other words, we want to investigate ideal number of subjects beyond which the difference between subject groups does not change substantially. Here, we investigate this question for all morphological measures and the Desikan-Killiany brain atlas as we used in the rest of the study.

We used 228 subjects from the Cam-CAN data set in a narrowed age range of 18-45. As we are interested in comparability (comparing different subject groups), we split the data in two distinct halves and calculate the structural covariance matrix for each half and obtain their difference. We repeat this process 1000 times using different splits to obtain a mean and standard deviation of the difference.

To assess the effect of number of subjects, we also repeat the above process systematically for different numbers of subjects in the halves we obtain. E.g. for 50 subjects, we have 50 distinct subjects in each half to compute the structural covariance matrix and their difference.

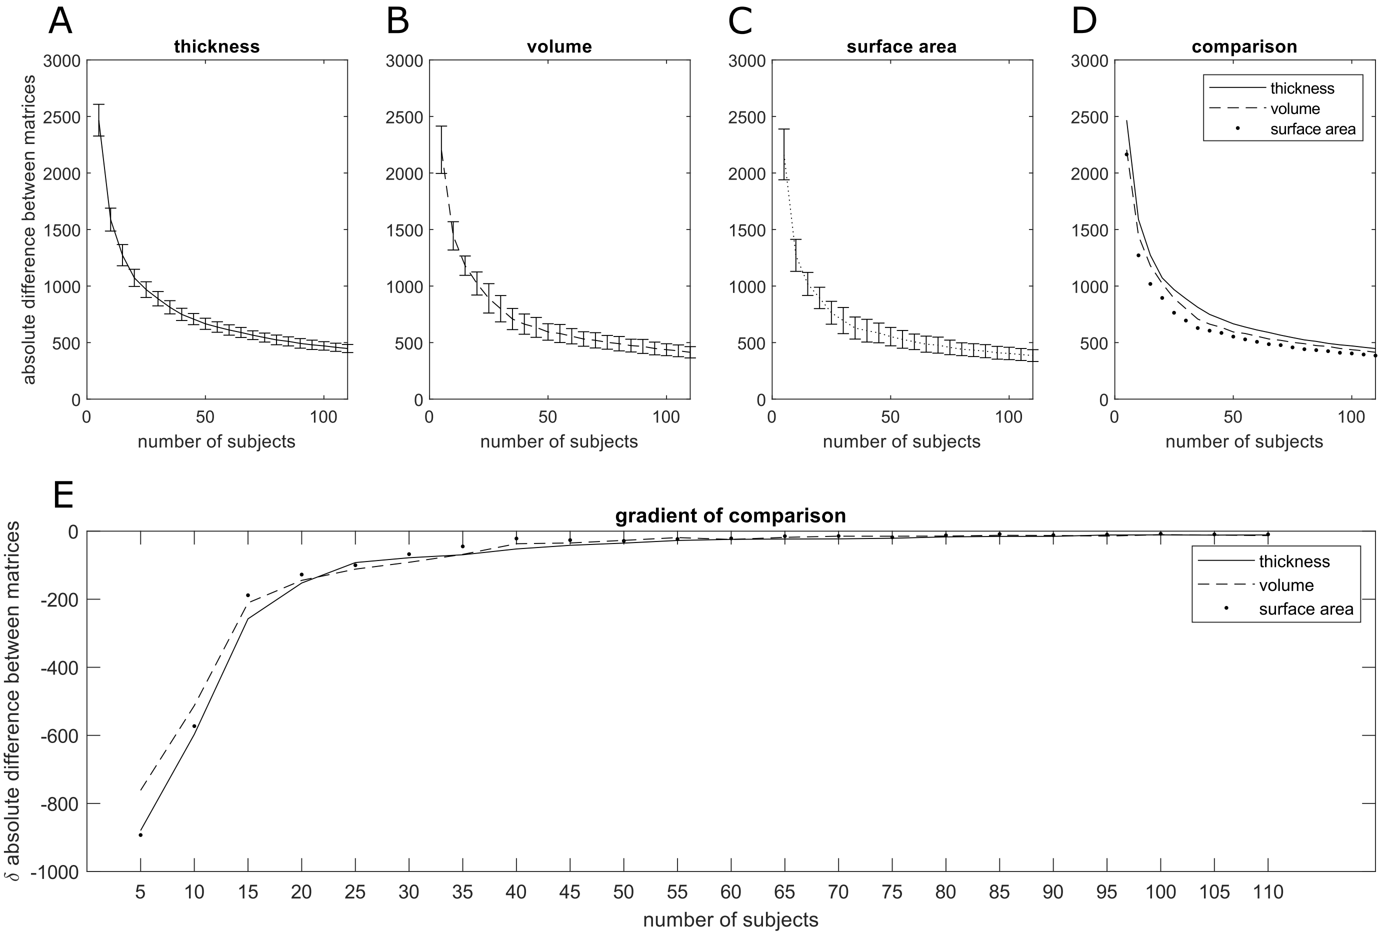


Figure S18: Effect of number of subjects on comparability. Panel (A)-(C) depict the mean and standard deviation of the absolute difference of the covariance matrices between two distinct subject groups over 1000 iterations. The x-axes show the corresponding number of subjects. Each of the panels display a different morphological measure. Panel (D) shows a comparison between the mean of the absolute differences of the different morphological measures. Panel (E) displays the gradient of the plots in (D)

Fig. S18 shows the mean and standard deviation of the differences plotted against the number of subjects. For all brain measures the difference between subject groups decreases with an increased number of subjects. However, beyond around 30 to 40 subjects the difference decreases less strongly which can be seen on the gradient depicted in panel (E). For more than approximately 60-80 subjects the difference does not decrease substantially anymore. We can also see that thickness is least comparable and surface area most comparable, consistent with our other analyses.

Our results indicate that, for the Desikan-Killiany atlas, we recommend to use n¿¿30 subjects for comparison between groups. We could also see that the difference between groups does not improve substantially beyond approximately 60-80 subjects. This further supports the number of subjects we used for our site comparison of the main results (86).

## 19. Effect of number of subjects on reliability

In Fig. S18 we could see that the comparability increases for a larger number of subjects. Here, we repeated the analysis for reliability for which we used the 45 subjects from the HCP scan-rescan data. We computed the structural covariance matrix for subjects of the scan data as well as for the same subjects of the rescan data and obtain the difference between the matrices. To calculate a mean and a standard deviation for each sample size, we subsampled the desired number of unique subjects over 1000 iterations, but maintained the same subjects in both scan and rescan groups for each iteration. As we only have 45 subjects, the number of possible subsamples naturally decreased as we increase our number of subjects up to 45. Hence the standard deviation is expected to drop rapidly with increased number of subjects, but this is a side effect of our limited sample size.

Fig. S19 shows that, also here, the difference between the scan and rescan matrices decreases with increasing number of subjects. As to be expected for our other results, these differences are lower in overall magnitude than for comparability (Fig. S18). Similar to before, beyond around 30 subjects the difference decreases less strongly. We can also observe a convergence-like behaviour as in Fig. S18, but we do not have sufficient overall number of subjects to make definitive conclusions.

All in all, we can see a similar effect of number of subjects like for comparability. The recommendation n¿¿30 subjects is also supported by these results. However, further studies with much larger single-site sample sizes are required to make definitive recommendations.

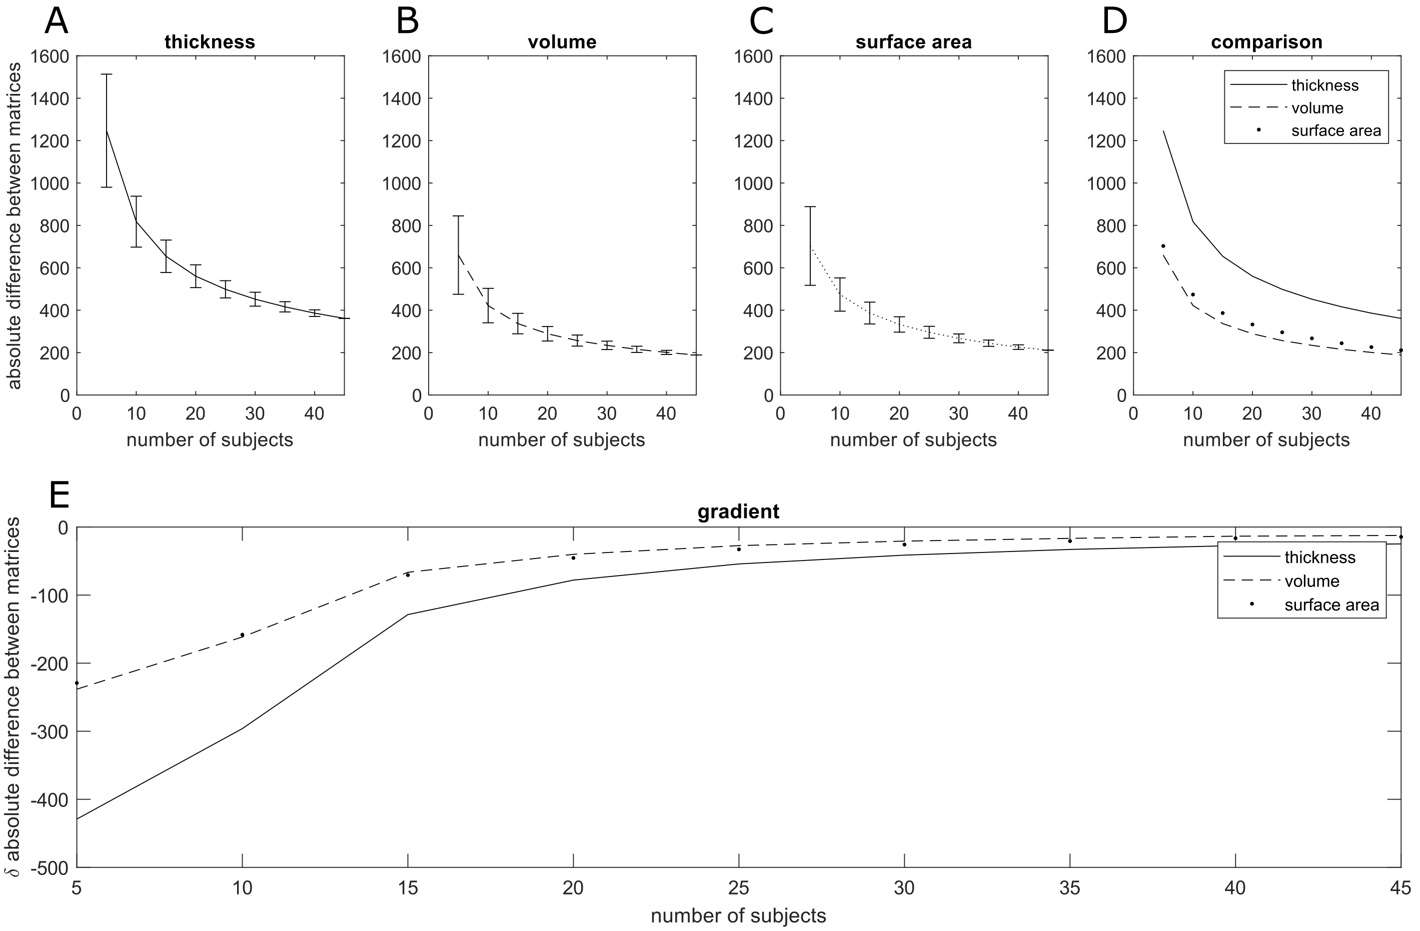


Figure S19: Effect of number of subjects on reliability. All plots are computed for the difference in structural covariance of HCP scan-rescan data. Panel (A)-(C) depict the mean and standard deviation of the absolute difference of the covariance matrices between the scan and rescan group over 1000 iterations. The x-axes show the corresponding number of subjects. Each of the panels display a different morphological measure. Panel (D) shows a comparison between the mean of the absolute differences of the different morphological measures. Panel (E) displays the gradient of the plots in (D)

## Additional references


[1] K. B. Nooner, S. Colcombe, R. Tobe, M. Mennes, M. Benedict, A. Moreno, L. Panek, S. Brown, S. Zavitz, Q. Li, et al., The nki-rockland sample: a model for accelerating the pace of discovery science in psychiatry, Frontiers in neuroscience 6 (2012) 152.
